# Supplementary material for: Prevalence of radio jets associated with galactic outflows and feedback from quasars
Source: arXiv:1902.07727 ancillary file (2019-02-20)
Supplement: Supplementary file 1 [file jarvis_radio_jets_paper_supplement.pdf]

# Supplementary information

This document provides more details on the *UV* to *FIR* SED fitting used in this work as well as a detailed presentation of our radio data and IFS data used for the analyses in the main paper. We also show additional radio and IFS data for two targets that were not included in the final primary sample (see Section 3.1).

## APPENDIX A: SED ANALYSIS

Here we describe the photometric data and SED fitting procedure used to derive stellar masses, AGN luminosities and far-infrared luminosities due to star formation presented in Section 2.2.

### A1 Photometry

We gathered archival data from the *UV* to *FIR* (0.1516–350 $\mu$m). In the *UV* we used data from The Galaxy Evolution Explorer (GALEX; far-*UV* at 1516Å and near-*UV* at 2267Å; Bianchi et al. 2014; Martin et al. 2005), and in the optical SDSS ($u$, $g$, $r$, $i$ and $z$ bands; Abolfathi et al. 2018). In the near infrared we took values from the Extended Source Catalogue of The Two Micron All Sky Survey (2MASS; J, H and $K_s$ bands Skrutskie et al. 2006)[1] , the Wide-field Infrared Survey Explorer (WISE) all-sky survey (3.4, 4.6, 12, and 22 $\mu$m Wright et al. 2010), and the Infrared Astronomical Satellite (IRAS; 12, 25, 60 and 100 $\mu$m Neugebauer et al. 1984) faint source catalogue (Moshir et al. 1992)[2]. We added in quadrature 30 per cent of the measured flux densities to the quoted WISE uncertainties to account for calibration uncertainties in the WISE data (Wright et al. 2010). Finally, where available we used data from the ESA *Herschel* Space Observatory (Pilbratt et al. 2010) using data from the PACS (Poglitsch et al. 2010) and SPIRE (Griffin et al. 2010) point source catalogues at 70, 100, 160 and 250, 350 $\mu$m respectively, in the far infrared.

For the WISE and 2MASS surveys we took the closest positional match to the SDSS position (all are < 2 arcsec). For GALEX we searched for all catalogue entries within 6.5 arcsec and took the detection with the lowest error in case of multiple observations (from the different GALEX surveys). For IRAS we followed a log likelihood method of matching IRAS to WISE counterparts to account for the large and asymmetric IRAS beam following Wang et al. (2014). For the sources that were observed by IRAS but that we were not able to obtain IRAS flux density measurements we estimated conservative maximum upper limits of 0.25, 0.4, 0.3, and 3 mJy for the 12, 25, 60, and 100 $\mu$m bands respectively.[3] Finally we applied corrections for galactic extinction to all photometry at wavelengths shorter than (and including) 2MASS, at which point the corrections are already smaller than the errors. Specifically, we used the Schlafly & Finkbeiner (2011) absorption values.[4]

### A2 SED fitting

In order to fit the SEDs we used the CIGALE code (version 0.12.0), which takes into account the energy balance between the absorption due to dust in the *UV*–optical regime and the corresponding re-emission in the *FIR*. The output parameters and their uncertainties are computed through a Bayesian statistical analysis: for each parameter of interest the code builds a probability distribution function (PDF) by summing the term $\exp(-\chi^2/2)$, associated to each model, in given bins of the parameter space. The procedure we applied and the input values we used closely follow Circosta et al. (2018), but we give some specific details here.

We modelled the stellar emission, which dominates the wavelength range 0.3–5 $\mu$m with the Bruzual & Charlot (2003) stellar population models, and assuming a delayed exponentially declining star formation history (SFH). The metallicity is fixed to solar (0.02) and the stellar population ages are constrained to be younger than the age of the Universe at the redshift of the targets. To account for attenuation we applied to the stellar contribution a modified version of the Calzetti et al. (2000) curve multiplied in the *UV* range by a power law with variable slope $\delta$. Negative slopes of the additional power law produce steeper attenuation curves and a slope equal to 0 reproduces the Calzetti et al. (2000) curve. Differential reddening undergone by young stars (<10 Myr) and old stars (>10 Myr) was taken into account by applying the reduction factor, $E(B-V)_{\rm old}/E(B-V)_{\rm young}$, fixed to 0.44.

The emission from dust heated by star formation, dominating the *FIR* regime, is reproduced using the library of Dale et al. (2014). We set the AGN contribution to these dust models equal to zero, in order to model the AGN emission separately using the models presented by Fritz et al. (2006). We only considered the AGN templates representative of type 2 AGN (see Circosta et al. 2018). Templates reproducing nebular emission from H II regions based on the models by Inoue (2011) were also included. We note that repeating the fits without nebular lines changes our output values of interest (see Table 2) by at most a factor of 1.3 with the stellar mass being the most effected.

[1] For J1338+1503, which was not in the Extended 2MASS source catalogue, we used the values from the point source catalogue.
[2] We also searched for significant detections using the SCANPI tool to inspect the data (http://irsa.ipac.caltech.edu/applications/Scanpi).
[3] One source (J1100+0846) falls into an area of the sky that was not observed by IRAS and we therefore cannot place photometric constraints on the IRAS bands for this source.
[4] https://irsa.ipac.caltech.edu/applications/DUST/

© 0000 The Authors

## APPENDIX B: ADDITIONAL FIGURES

In this section we provide three sets of figures to present our data and analyses for each of the primary targets (Fig. B1–B30) as follows:

(i) The first set of figures shows the radio images used for calculating the spectral index for each feature we identified (see Section 4.1.1). Alongside, we show the Gaussian model fits (and data−model residuals) used to calculate the flux densities from the images. We also show the radio SEDs for each feature. Table B1 gives the details of how each of these radio images was constructed and the corresponding properties of the synthesised beams and noise (see Section 3.1.2). Finally, we show the broad-band *UV*-to-*FIR* SEDs used to calculate stellar masses, star-formation rates and AGN luminosities (see Section 2.2).

(ii) The second set of figures compares the SDSS or when available, *HST* imaging, ionized gas kinematics from our IFS data, and the radio morphologies to complement the discussion presented in Section 5.3. We also show [O III] emission-line profiles extracted from our IFS data at locations of interest motivated by the ionized gas and radio features observed. When numbers are quoted in relation to the [O III] kinematics in the main manuscript they are taken from, or motivated by, the line profiles shown in these figures. These figures also show the non-parametric kinematic maps extracted from the IFS data (see Section 4.2). When we have both VIMOS and GMOS data for a target we show the maps derived from both sets of data.

(iii) The final set of figures for each target presents narrow-band images from the IFS data, stepping through various wavelength slices (optionally in an animated format) to further highlight how different velocity components of the ionized gas relate to the radio features seen. Video formats of these figures are also included as separate .mp4 files with this supplementary information.

## APPENDIX C: NON-PRIMARY SAMPLE

From our incomplete 16A-182 VLA run we obtained C-band B-configuration data for two quasar targets not included in the primary sample (see Section 3.1). These data are presented here (Fig. C1) and are briefly discussed in the figure caption.

## REFERENCES


Abolfathi B., et al., 2018, The Astrophysical Journal Supplement Series, 235, 42
Bianchi L., Conti A., Shiao B., 2014, Advances in Space Research, 53, 900
Bruzual G., Charlot S., 2003, MNRAS, 344, 1000
Calzetti D., Armus L., Bohlin R. C., Kinney A. L., Koornneef J., Storchi-Bergmann T., 2000, ApJ, 533, 682
Circosta C., et al., 2018, A&A, 620, A82
Comerford J. M., Pooley D., Barrows R. S., Greene J. E., Zakamska N. L., Madejski G. M., Cooper M. C., 2015, ApJ, 806, 219
Cui J., Xia X.-Y., Deng Z.-G., Mao S., Zou Z.-L., 2001, AJ, 122, 63
Dale D. A., Helou G., Magdis G. E., Armus L., Díaz-Santos T., Shi Y., 2014, ApJ, 784, 83
Fritz J., Franceschini A., Hatziminaoglou E., 2006, MNRAS, 366, 767
Gallimore J. F., Axon D. J., O'Dea C. P., Baum S. A., Pedlar A., 2006, AJ, 132, 546
Greene J. E., Zakamska N. L., Smith P. S., 2012, ApJ, 746, 86
Griffin M. J., et al., 2010, A&A, 518, L3
Harrison C. M., Alexander D. M., Mullaney J. R., Swinbank A. M., 2014, MNRAS, 441, 3306
Harrison C. M., Thomson A. P., Alexander D. M., Bauer F. E., Edge A. C., Hogan M. T., Mullaney J. R., Swinbank A. M., 2015, ApJ, 800, 45
Heesen V., Croston J. H., Harwood J. J., Hardcastle M. J., Hota A., 2014, MNRAS, 439, 1364
Hogan M. T., et al., 2015, MNRAS, 453, 1201
Inoue A. K., 2011, MNRAS, 415, 2920
Keel W. C., et al., 2015, AJ, 149, 155
Kharb P., O'Dea C. P., Baum S. A., Colbert E. J. M., Xu C., 2006, ApJ, 652, 177
Lansbury G. B., Jarvis M. E., Harrison C. M., Alexander D. M., Del Moro A., Edge A. C., Mullaney J. R., Thomson A. P., 2018, ApJ, 856, L1
Martin D. C., et al., 2005, ApJ, 619, L1
Moshir M., Kopman G., Conrow T. A. O., 1992, IRAS Faint Source Survey, Explanatory supplement version 2
Neugebauer G., et al., 1984, ApJ, 278, L1
Orienti M., 2016, Astronomische Nachrichten, 337, 9
Orienti M., Dallacasa D., 2014, MNRAS, 438, 463
Pilbratt G. L., et al., 2010, A&A, 518, L1
Poglitsch A., et al., 2010, A&A, 518, L2
Schlafly E. F., Finkbeiner D. P., 2011, ApJ, 737, 103
Skrutskie M. F., et al., 2006, AJ, 131, 1163
Sun A.-L., Greene J. E., Zakamska N. L., Nesvadba N. P. H., 2014, ApJ, 790, 160
Villar-Martín M., Cabrera-Lavers A., Humphrey A., Silva M., Ramos Almeida C., Piqueras-López J., Emonts B., 2018, MNRAS, 474, 2302
Wang L., Rowan-Robinson M., Norberg P., Heinis S., Han J., 2014, MNRAS, 442, 2739
Wright E. L., et al., 2010, AJ, 140, 1868


This paper has been typeset from a TEX/LATEX file prepared by the author.

**Table B1.** Summary of radio images shown in this supplementary material
Notes: For each target (name in column 1) and for each of the resolution matched images created for measuring flux densities (figure number, resolution and frequency given in columns 2, 3 and 4), the synthesised beams and noise are given (columns 5-7), as well as the noise level (7). (8) describes the measurement set used, where C-A indicates a VLA C-band A-configuration image (etc.). 'C-A + C-B' means a concatenation of the C-band A and B-configuration data was used with relative weighting of 4:1; (9) describes the weighting scheme used to image the data. The last two rows, separated by a line, give the details for the two VLA images shown in Appendix C for the sources not in our primary sample.

| Name | Fig. | res. | Frq. (GHz) | Beam HPBW (arcsec) | Beam PA (deg) | Noise ($\mu$Jy/beam) | Data | Weighting |
|---|---|---|---|---|---|---|---|---|
| (1) | (2) | (3) | (4) | (5) | (6) | (7) | (8) | (9) |
| J0945+1737 | Fig. B1 | HR | 1.5 | 0.23×0.23 | 31 | 254 | e-MERLIN | |
| | | HR | 5.2 | 0.26×0.26 | -32 | 29 | C-A | uniform |
| | | HR | 7.2 | 0.22×0.2 | -16 | 20 | C-A | briggs 0.0 |
| | | LR | 1.5 | 1.59×1.11 | 68 | 77 | L-A | briggs 0.5 |
| | | LR | 5.2 | 1.52×1.3 | 43 | 17 | C-A + C-B | natural & 160 k$\lambda$ taper |
| | | LR | 7.2 | 1.45×1.31 | 47 | 16 | C-A + C-B | natural & 120 k$\lambda$ taper |
| J0958+1439 | Fig. B4 | HR | 1.5 | 0.23×0.21 | -27 | 319 | e-MERLIN | |
| | | HR | 5.2 | 0.27×0.26 | -50 | 18 | C-A | uniform |
| | | HR | 7.2 | 0.23×0.21 | -19 | 13 | C-A | briggs 0.0 |
| | | LR | 1.5 | 1.73×1.11 | 64 | 30 | L-A | briggs 0.5 |
| | | LR | 5.2 | 1.48×1.23 | 45 | 10 | C-A + C-B | natural & 200 k$\lambda$ taper |
| | | LR | 7.2 | 1.36×1.14 | 45 | 9 | C-A + C-B | natural & 150 k$\lambda$ taper |
| J1000+1242 | Fig. B7 | HR | 1.5 | 0.27×0.22 | -40 | 227 | e-MERLIN | |
| | | HR | 5.2 | 0.28×0.26 | -20 | 34 | C-A | uniform |
| | | HR | 7.2 | 0.27×0.24 | -8 | 27 | C-A | briggs 0.6 |
| | | LR | 1.5 | 1.63×1.12 | 63 | 48 | L-A | briggs 0.5 |
| | | LR | 5.2 | 1.45×1.14 | 23 | 21 | C-A + C-B | natural & 200 k$\lambda$ taper |
| | | LR | 7.2 | 1.31×1.16 | 40 | 21 | C-A + C-B | natural & 140 k$\lambda$ taper |
| J1010+1413 | Fig. B10 | HR | 1.5 | 0.24×0.22 | -11 | 156 | e-MERLIN | |
| | | HR | 5.2 | 0.27×0.26 | -47 | 19 | C-A | uniform |
| | | HR | 7.2 | 0.24×0.22 | -14 | 13 | C-A | briggs 0.2 |
| | | LR | 1.5 | 1.55×0.83 | 84 | 79 | L-A | uniform |
| | | LR | 5.2 | 1.32×1.19 | 44 | 13 | C-A + C-B | natural & 200 k$\lambda$ taper |
| | | LR | 7.2 | 1.29×1.09 | 46 | 9 | C-A + C-B | natural & 160 k$\lambda$ taper |
| J1010+0612 | Fig. B13 | HR | 1.5 | 0.32×0.18 | 25 | 3438 | e-MERLIN | |
| | | HR | 5.2 | 0.3×0.28 | -54 | 89 | C-A | uniform |
| | | HR | 7.2 | 0.22×0.2 | -69 | 87 | C-A | uniform |
| | | LR | 1.5 | 1.99×0.9 | 59 | 508 | L-A | briggs 0.5 |
| | | LR | 5.2 | 1.57×1.11 | 48 | 60 | C-A + C-B | natural & 200 k$\lambda$ taper |
| | | LR | 7.2 | 1.5×1.12 | 46 | 51 | C-A + C-B | natural & 150 k$\lambda$ taper |
| J1100+0846 | Fig. B16 | HR | 1.5 | 0.3×0.18 | 26 | 549 | e-MERLIN | |
| | | HR | 5.2 | 0.28×0.27 | -35 | 53 | C-A | uniform |
| | | HR | 7.2 | 0.25×0.22 | -20 | 50 | C-A | briggs 0.2 |
| | | LR | 1.5 | 1.57×1.12 | 61 | 109 | L-A | briggs 0.5 |
| | | LR | 5.2 | 1.54×1.29 | 37 | 33 | C-A + C-B | natural & 160 k$\lambda$ taper |
| | | LR | 7.2 | 1.27×1.12 | 39 | 36 | C-A + C-B | natural & 150 k$\lambda$ taper |
| J1316+1753 | Fig. B19 | HR | 1.5 | 0.3×0.17 | 27 | 136 | e-MERLIN | |
| | | HR | 5.2 | 0.32×0.27 | 78 | 20 | C-A | uniform |
| | | HR | 7.2 | 0.25×0.22 | -70 | 13 | C-A | briggs 0.0 |
| | | LR | 1.5 | 1.16×1.06 | 20 | 28 | L-A | briggs 0.5 |
| | | LR | 5.2 | 1.16×1.13 | -28 | 12 | C-A + C-B | natural & 200 k$\lambda$ taper |
| | | LR | 7.2 | 1.12×1.07 | 30 | 10 | C-A + C-B | natural & 160 k$\lambda$ taper |
| | | LR | 5.2 | 1.0×0.92 | 43 | 13 | C-B | uniform |
| | | LR | 7.2 | 0.93×0.83 | 54 | 7 | C-B | briggs 0.6 |
| J1356+1026 | Fig. B25 | HR | 1.5 | 0.32×0.17 | 24 | 570 | e-MERLIN | |
| | | HR | 5.2 | 0.35×0.29 | -83 | 86 | C-A | uniform |
| | | HR | 7.2 | 0.27×0.23 | -69 | 88 | C-A | briggs 0.0 |
| | | LR | 1.5 | 1.18×1.06 | 21 | 97 | L-A | briggs 0.5 |
| | | LR | 5.2 | 1.3×0.99 | -1 | 32 | C-A + C-B | natural |
| | | LR | 7.2 | 1.19×1.02 | -178 | 32 | C-A + C-B | natural & 200 k$\lambda$ taper |
| J1430+1339 | Fig. B28 | HR | 1.5 | 0.31×0.16 | 24 | 205 | e-MERLIN | |
| | | HR | 5.2 | 0.4×0.28 | -84 | 32 | C-A | uniform |
| | | HR | 7.2 | 0.32×0.24 | -71 | 22 | C-A | briggs 0.2 |
| | | LR | 1.5 | 1.15×1.06 | 13 | 42 | L-A | briggs 0.5 |
| | | LR | 5.2 | 1.22×1.16 | 52 | 15 | C-A + C-B | briggs 0.5 & 120 k$\lambda$ taper |
| | | LR | 7.2 | 1.18×1.1 | 71 | 14 | C-A + C-B | briggs 0.5 & 100 k$\lambda$ taper |
| J1355+1300 | Fig. C1 | LR | 6.2 | 1.01×0.92 | 43 | 6 | C-B | briggs 0.5 |
| J1504+0151 | Fig. C1 | LR | 6.2 | 0.85×0.78 | 60 | 12 | C-B | uniform |

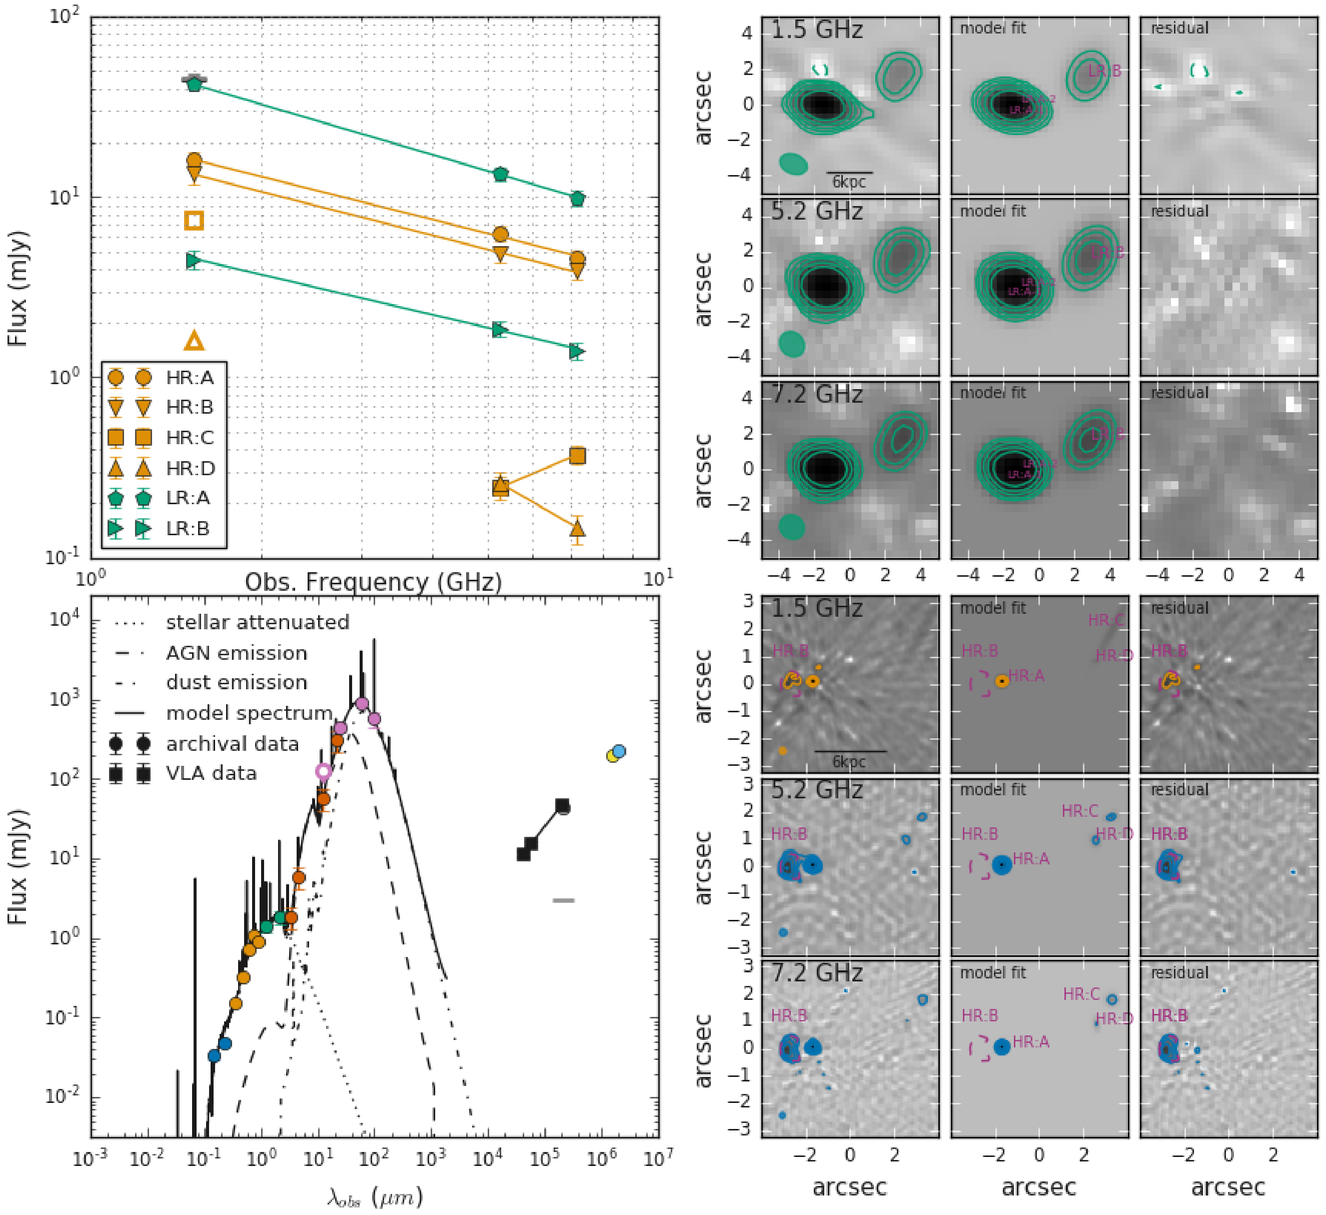


**Figure B1.** Broadband SED, multi-frequency radio images including model fits, and the radio SEDs for the individual radio features in J0945+1737. The data points in the broadband SED (bottom left) are colour coded by instrument / survey and the various components of the fits are shown by different styled lines, as in Fig. 4. The radio SED (top left) shows the flux densities for each morphological component marked by a distinct symbol, with the high resolution (HR) components in orange and the low-resolution (LR) components in green. The FIRST and NVSS fluxes (galaxy integrated) are also shown in black and grey, respectively. For both the radio and *UV-FIR* SEDs, upper limits are represented by open symbols, while detections are filled. The multi-frequency radio images, Gaussian fits and model−data residuals are shown as the remaining columns with the LR images as the top three rows and the HR on the bottom three rows. The colour coding, contour levels and the morphological component labels are the same as in Fig. 5, with additional labels for the individual LR Gaussians components when multiple Gaussians were used. The scale bar (shown in the bottom of the 1.5 GHz image at each resolution) represents 6 kpc. For this source, in our high resolution images, we observe a nuclear component (HR:A) and jet/lobe structure to the east (HR:B). In the e-MERLIN image HR:B has the appearance of a bent jet. We note that LR:B, which we interpret as a second jet/lobe to the east, is mostly resolved out in the high resolution images, except for two very weak (HR:C and HR:D) features with uncertain flux density measurements and an unclear interpretation (see Fig. B2).

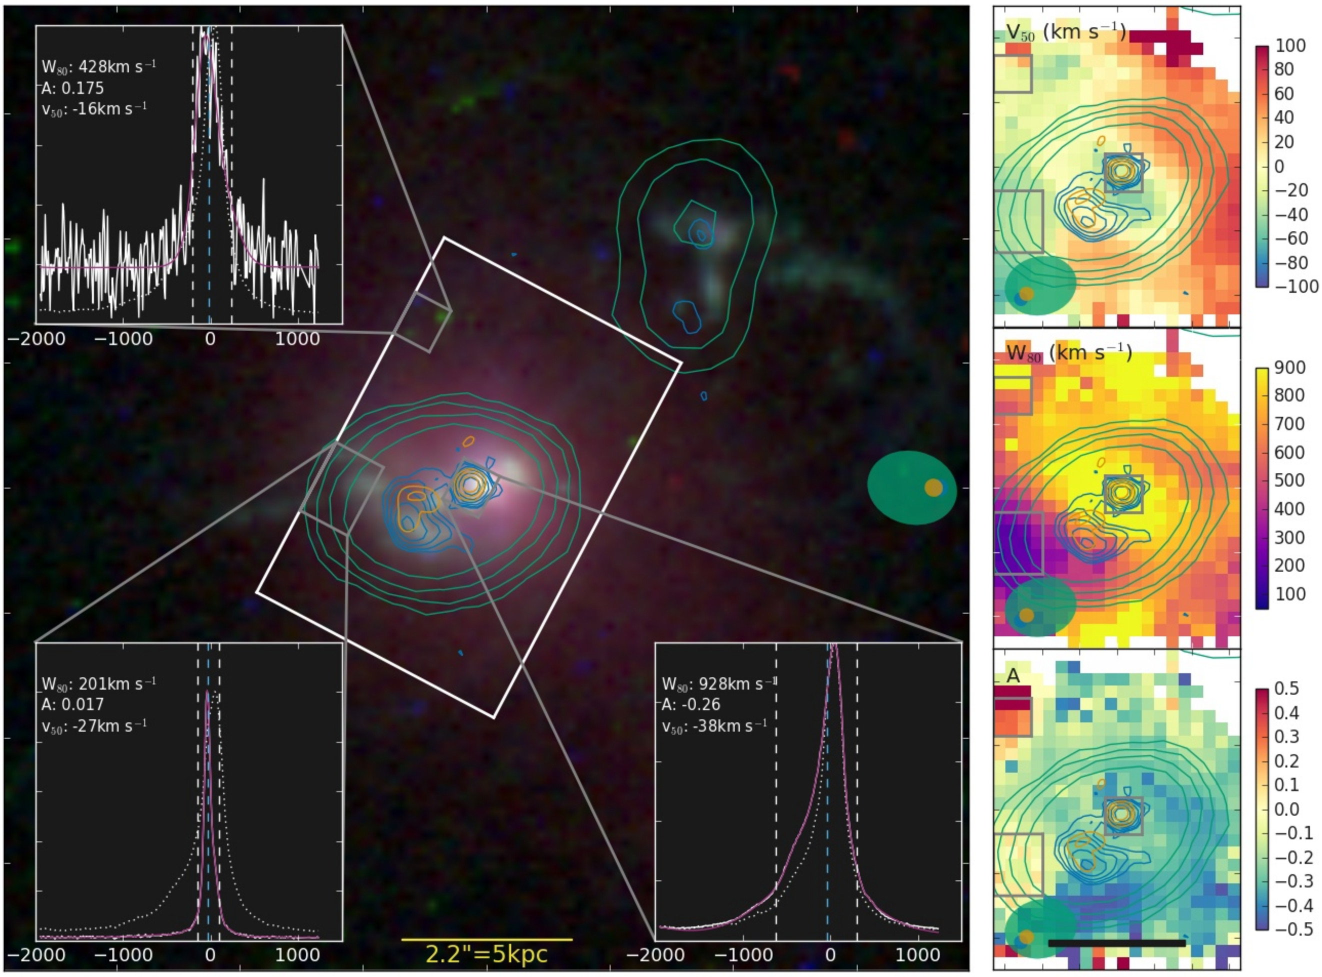


**Figure B2.** A comparison of the broad-band image, ionized gas and radio features for J0945+1737. The panel on the left shows the radio contours from Fig. 5 colour coded as they are in that figure with the synthesised beams represented by ellipses in the middle right of the figure. The background three-colour image is from archival HST data; with continuum from the F814W filter in red (Cui et al. 2001), [O III] and H$\beta$ narrow-band image from the FR551N filter in green, and H$\alpha$+[N II] narrow-band image from the FR716N filter in blue (observing proposal id.13741). The FOV of the GMOS IFS observations is overlaid in white. [O III] emission-line profiles are extracted from the regions of the data shown in grey boxes and are plotted in their respective corners. The weighted average of the pixels included is shown in white with the fit in magenta and the total spectra across the cube is shown as a dotted white curve for reference. The vertical white dashed lines mark $v_{10}$ and $v_{90}$ with the light-blue dashed line showing $v_{50}$, which is also written, along with the $W_{80}$ and asymmetry ($A$) for the extracted emission-line profile in the top left of each inset (see Section 4.2 for definitions). The second column shows the maps of $v_{50}$, $W_{80}$ and $A$ with the boxes used for the extracted spectrum overlaid, the scale bar in the asymmetry plot the same as in the main panel. As can be seen from the *HST* data, LR:B is coincident to a line emission dominated region and therefore it is likely related to the host galaxy. We propose that it is a secondary jet/lobe. The GMOS data reveals a bright, narrow, largely symmetric [O III] region just beyond HR:B, and we suggest that this kinematically distinct [O III] region has deflected the jet. The lack of an alignment between the positional angle of the two jet/lobes (LR:B and HR:B), and the differences in their distance to the probable core (HR:A), suggests that these could be due to multiple episodes of jet activity (see e.g., Kharb et al. 2006; Gallimore et al. 2006; Orienti 2016).

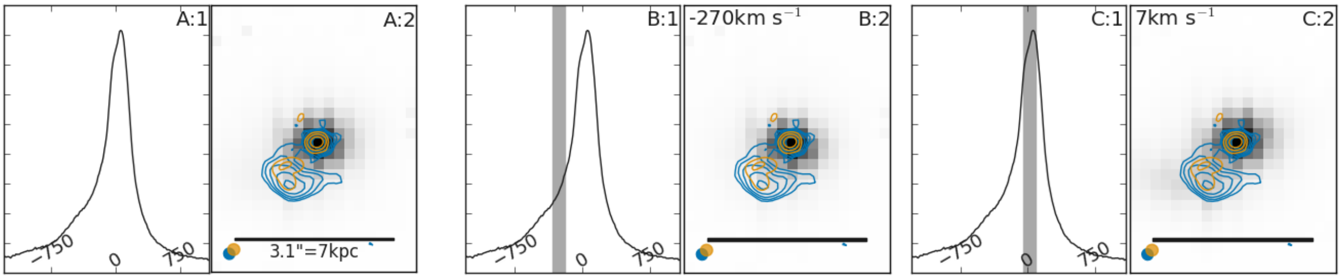


**Figure B3.** A:1: The total [O III] emission line profile of J0945+1737 across all spaxels, with wavelength given in km s$^{-1}$. A:2: an image from the IFS data, created by summing over the entire emission-line profile in A:1 for each spaxel. Radio contours from Fig. 5 are over-plotted, colour coded as in that figure. Panels B and C show individual wavelength slices, with sub-panel 1 showing the total [O III] emission-line profile with a grey bar marking the wavelength range over which the [O III] image in panel 2 is summed. The central velocity of each slice is shown in the top left corner of panel 2. In each image the synthesised beams are represented with ellipses in the bottom left. For this source, the slice shown in panel C (~7km s$^{-1}$) shows the distinct kinematic component associated with HR:B.
*In Adobe or other pdf readers with flash capabilities, this figure is a* click activated *video and panel A:2 steps through velocity slices from the wavelength ranges shown by the grey bar in panel A:1. The video file is also available separately.*

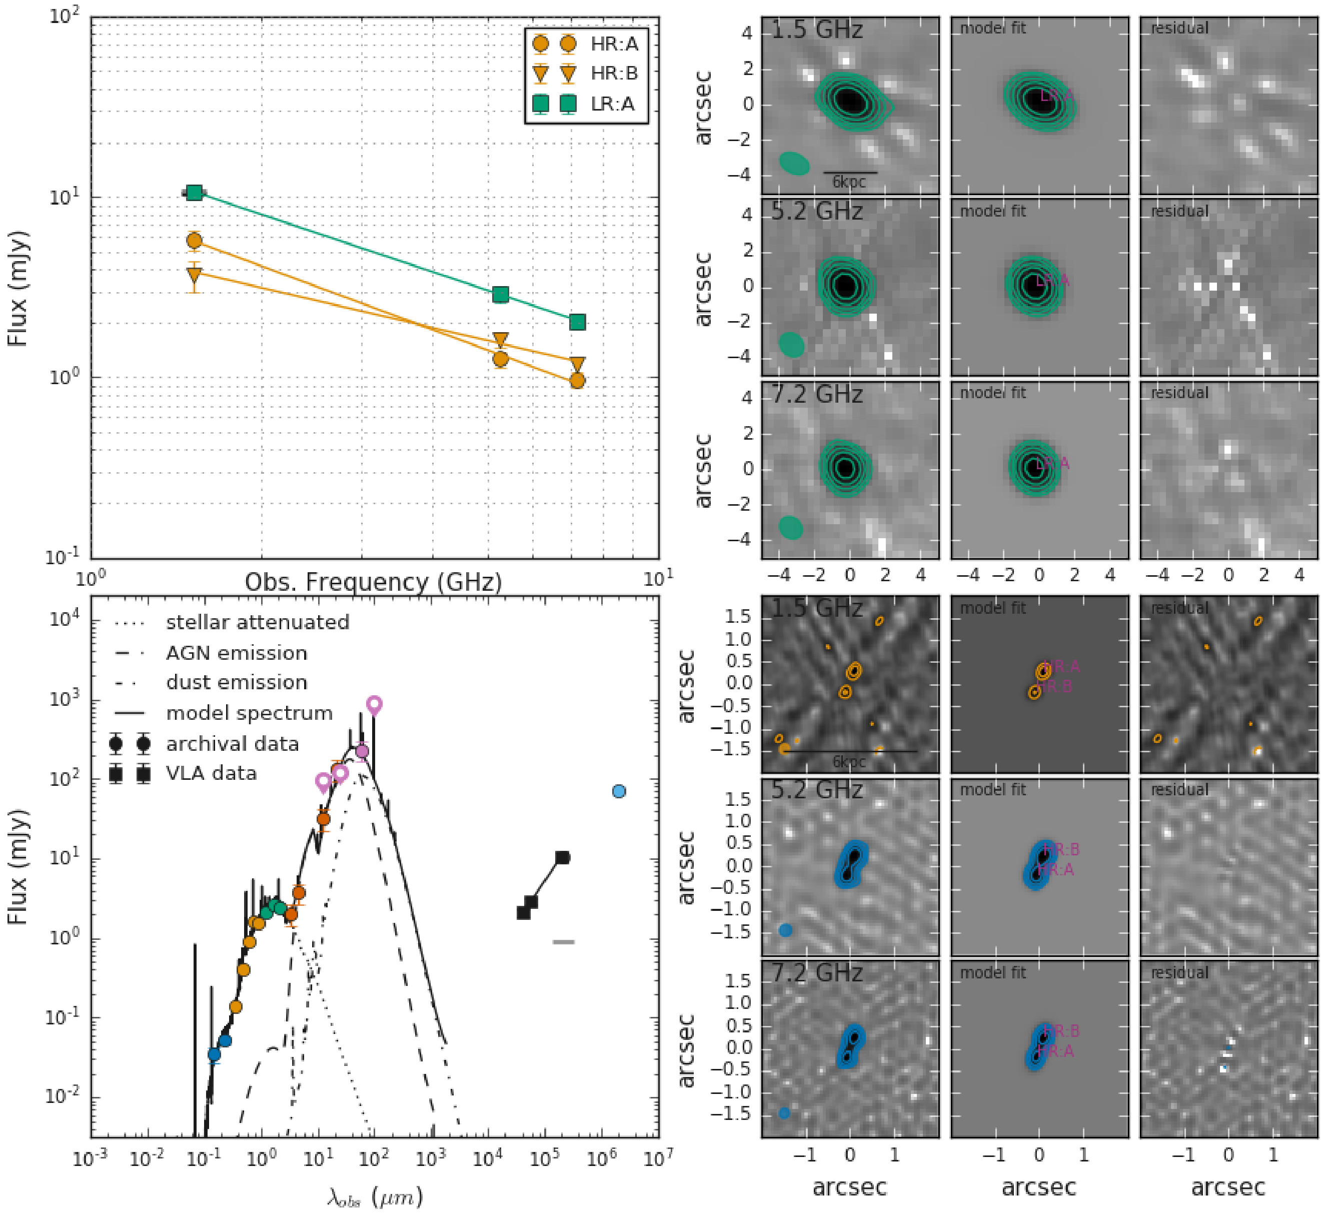


**Figure B4.** Same as Fig. B1 but for J0958+1439. In the high resolution images this source is resolved into two steep spectrum ($\alpha \sim -0.9$) components which we interpret as roughly symmetric radio lobes around an undetected central AGN core.

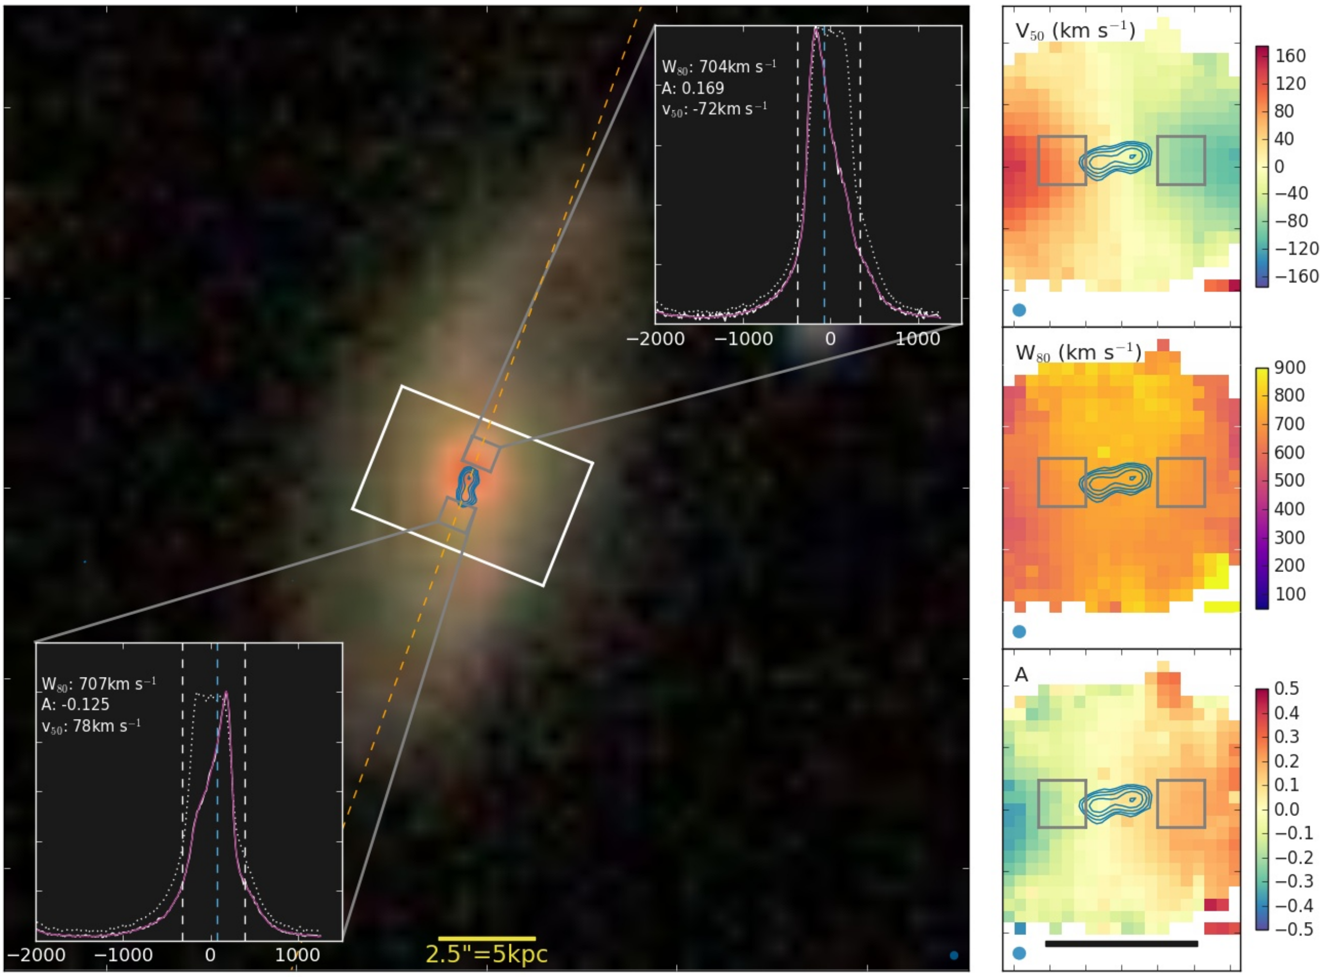


**Figure B5.** As Fig. B2 but for J0958+1439. Since there is no *HST* data for this source the SDSS three-colour image is used instead, as in Fig. 2. The orange dashed line marks the approximate direction of the velocity gradient from our [O III] measurements, which additionally, by eye, lies in the plane of the galactic disc. This means that the jet axis defined between HR:A and HR:B is into the galactic disc. At the location of each radio lobe we see a high-velocity ($\approx\pm75$ km s$^{-1}$) ionized gas component, as can be seen from the inset emission-line profiles.

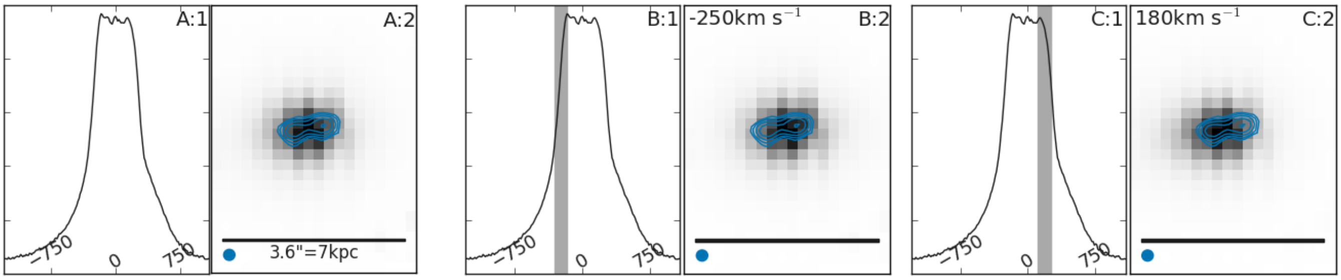


**Figure B6.** As Fig. B3 but for J0958+1439.

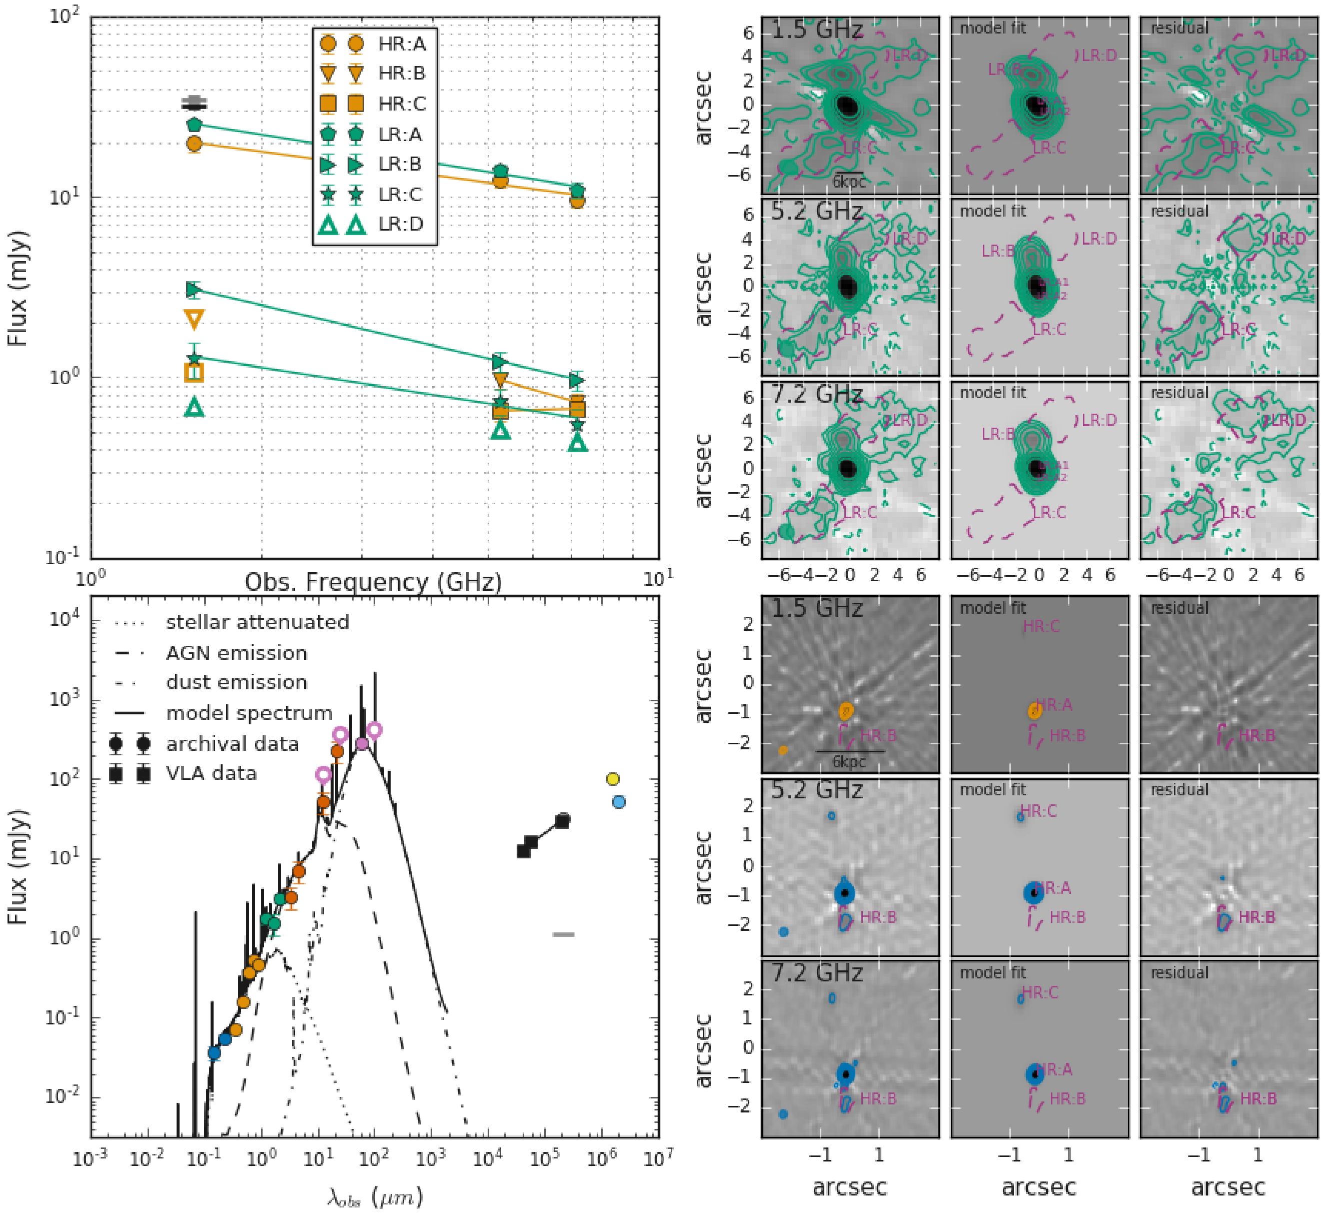


**Figure B7.** Same as Fig. B1 but for J1000+1242. We interpret the radio features in this source as jet/lobe structures with a flat spectrum hot spot (HR:C; $\alpha$ = 0.1) embedded in one of the lobes (LR:B). Furthermore, LR:C and LR:D are likely signs of deflection (see e.g., Heesen et al. 2014). HR:A, with a relatively flat spectral index of -0.4, most likely contains the radio core and possibly unresolved jet or lobe components. HR:B appears to be a jet. The GLEAM and TGSS data for this source (see bottom left panel) suggest that its radio spectrum turns over somewhere between 1.4 and 0.15 GHz, which, following the turnover - size relation from CSS/GPS sources (Orienti & Dallacasa 2014) corresponds to a size from 0.2–9kpc, consistent with the HR total size given in Table 4.

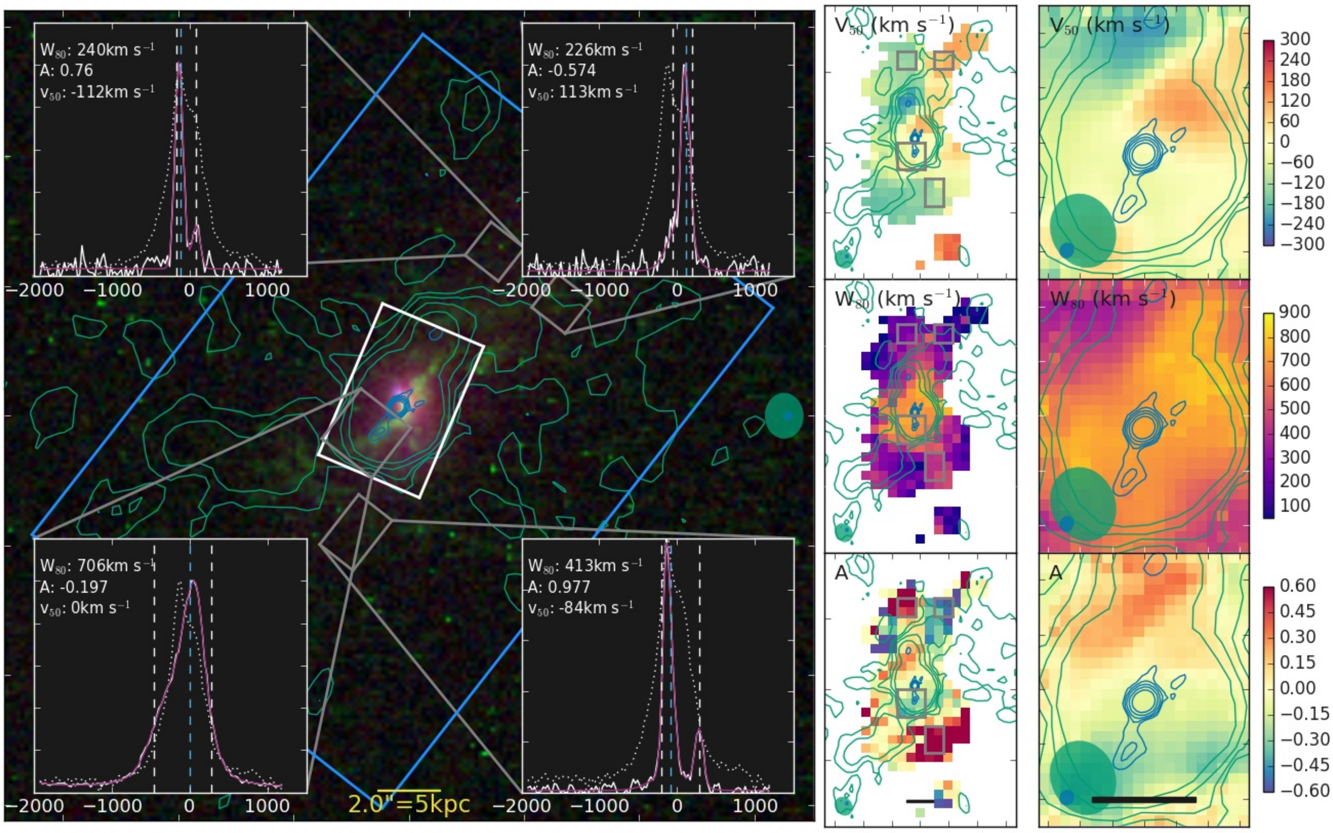


**Figure B8.** As Fig. B2 but for J1000+1242. The background three-colour image is from archival HST data (observing proposal id.14730), with IR continuum from the F160W filter in red, optical continuum from the F621M filter in blue and [O III] from the FQ575N filter in green. The VIMOS data is also shown as the middle column with the area covered by the displayed kinematics maps shown on the main image in light blue. The extracted emission-line profiles in the main panel are from the VIMOS data. Both the radio morphology and [O III] kinematics for this source are complex. Most notable is the line splitting shown in the lower right [O III] emission-line profile and by the high positive asymmetry in the same region, which we show to be due to a ∼10 kpc scale outflowing bubble (see Fig. 11; also see in Fig. B9). The HST data show that [O III] is enhanced along the southern jet and possibly along a corresponding northern jet, which is not observed in our radio images.

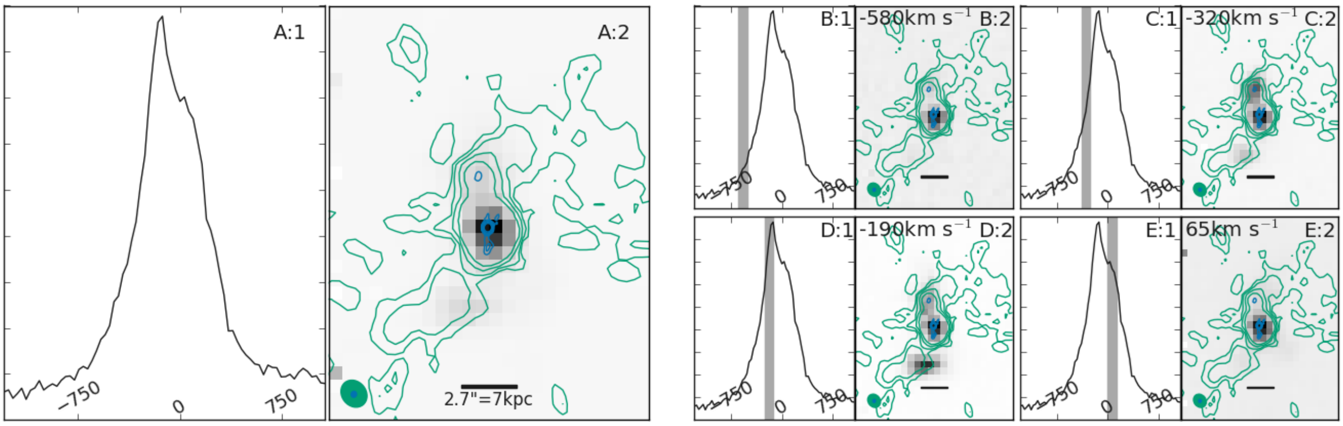


**Figure B9.** As Fig. B3 but for J1000+1242. Panels C and D show that the southern radio features are associated with kinematically distinct regions of ionized gas.

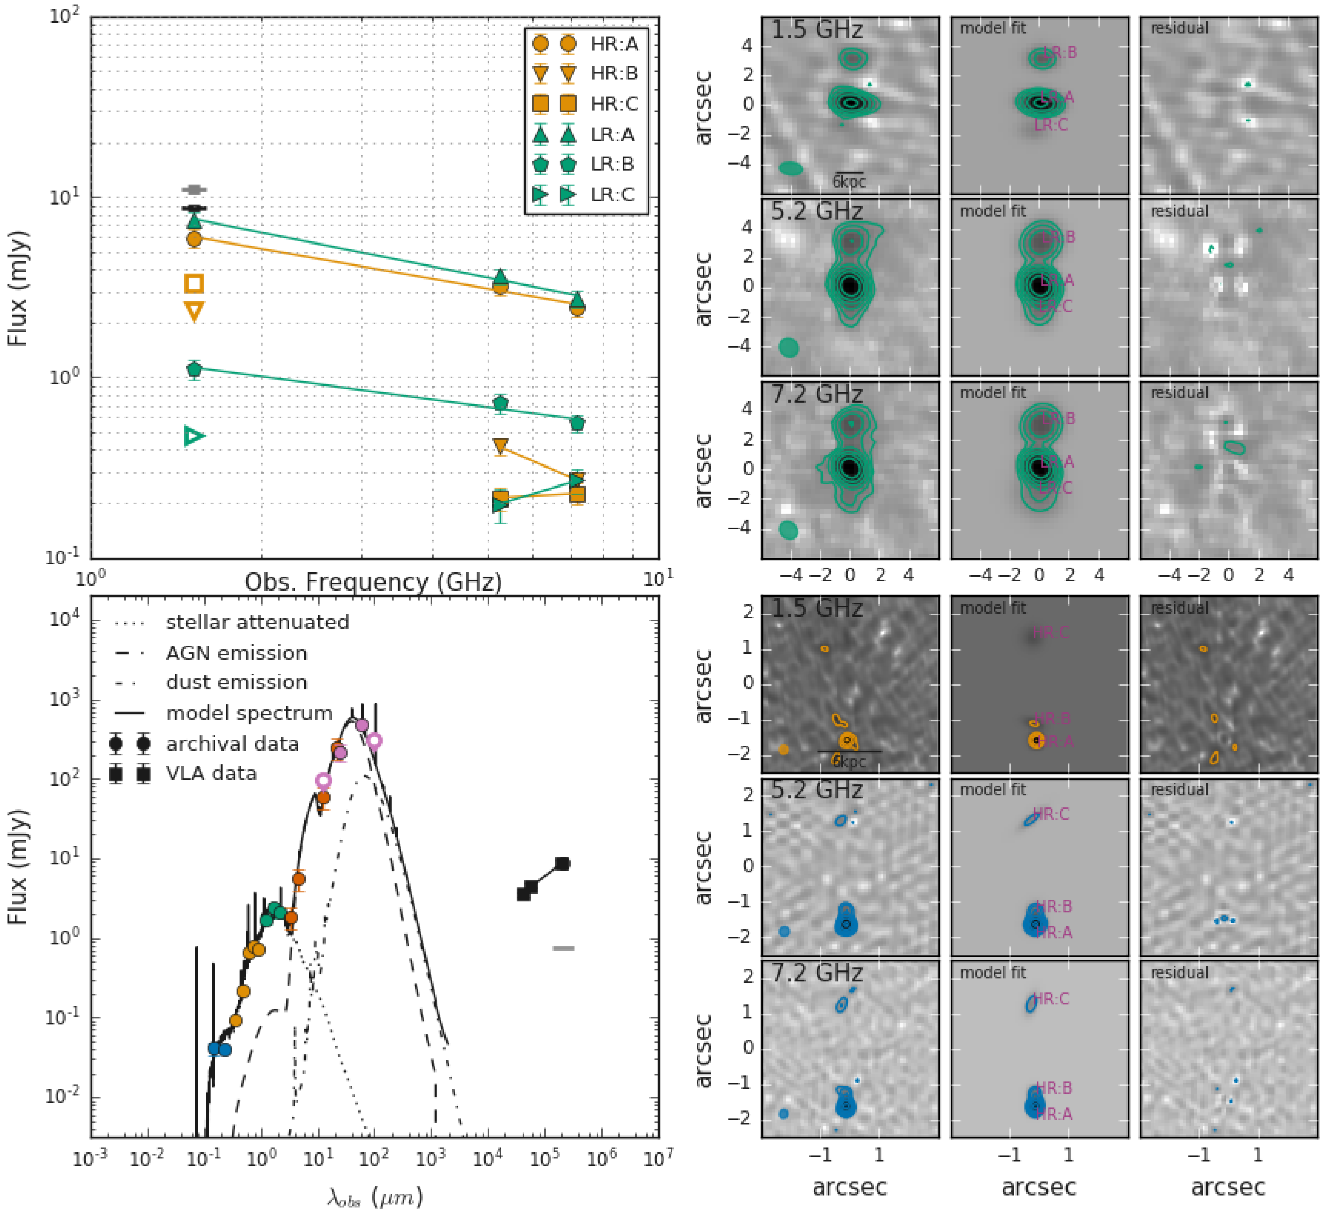


**Figure B10.** Same as Fig. B1 but for J1010+1413. The morphology of this source suggests a simple lobe (LR:B and LR:C) core structure with HR:C (with a relatively flat spectral index of $\alpha = 0.2$) as a hot spot and HR:B the base of the jet. The steepness ($\alpha = -0.6$) of HR:A however makes it difficult to identify as being dominated by an AGN core, possibly suggesting the presence of unresolved jet / lobe / wind features.

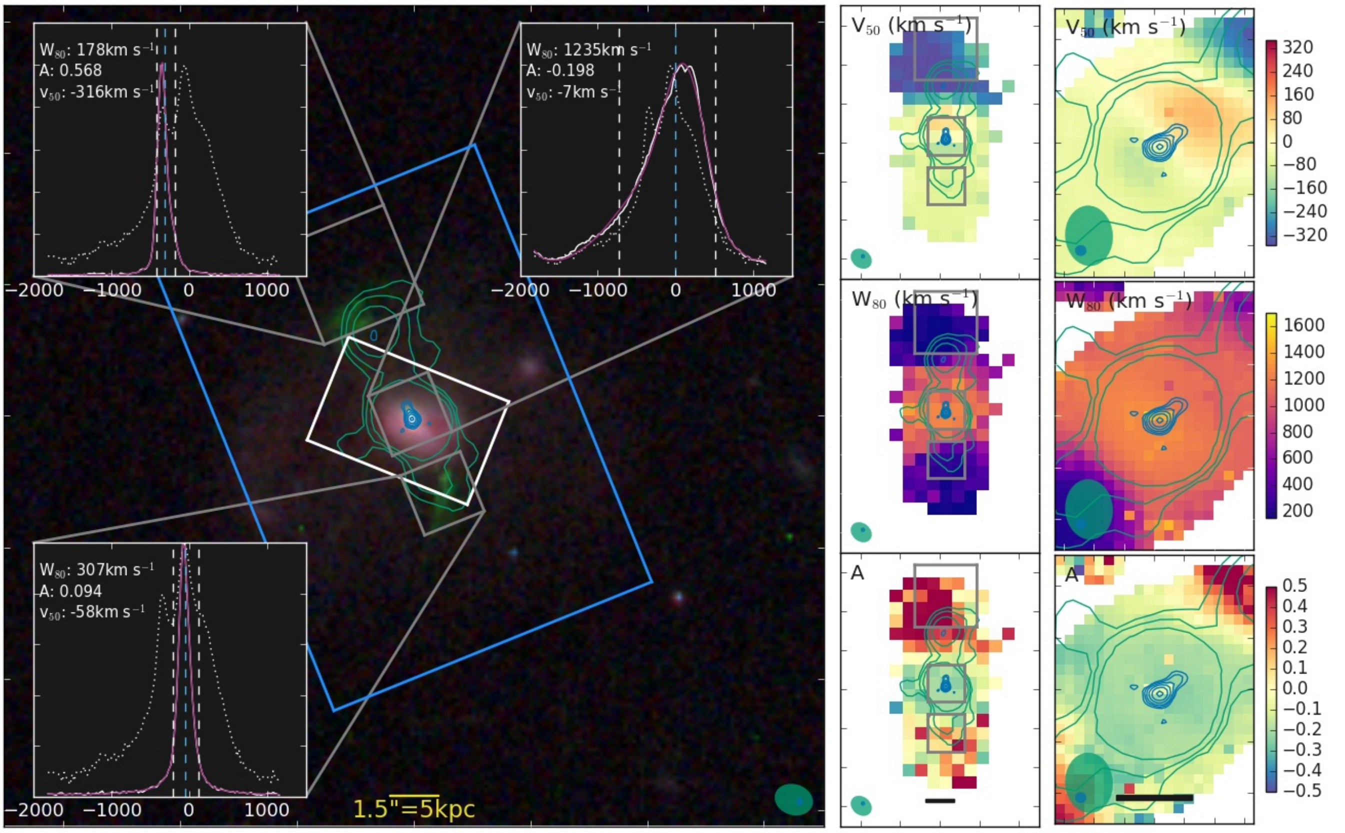

**Figure B11.** As Fig. B2 but for J1010+1413. The background three-colour image is from archival HST data (observing proposal id.14730), with IR continuum from the F160W filter in red, optical continuum from the F689M filter in blue and [O III] from the F621M filter in green. The VIMOS data is also shown as the middle column with the area covered by the kinematic maps derived from the VIMOS data shown on the main image in light blue. The extracted emission-line profiles are from the VIMOS data. The [O III] profile at the base of the jet (around HR:A and HR:B) is wide with a blue wing, indicative of outflows. The gas just beyond the extent of LR:B and LR:C is narrow and in both cases slightly blue shifted with respect to the peak central. For the gas in the north in particular this kinematically distinct [O III] feature could be responsible for the jet bending tentatively seen in HR:C and jet-gas interactions could be the cause of the velocity offset. Similarly, the southern jet could be truncated by the bright [O III] feature in the south, seen most clearly in the HST data.

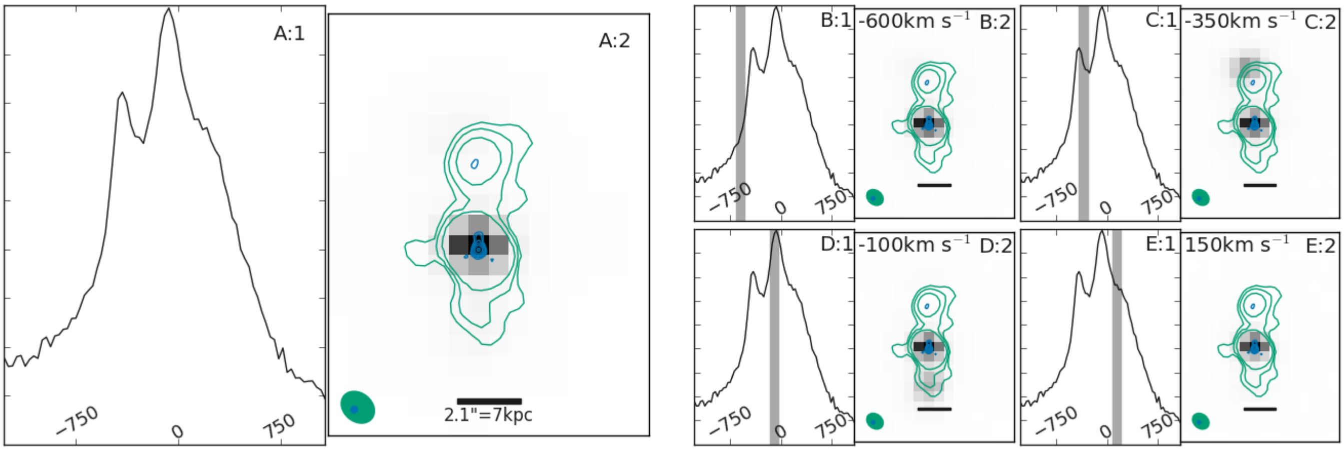

**Figure B12.** As Fig. B3 but for J1010+1413. The two main peaks seem to be associated with LR:B and LR:C (highlighted in panels C and D) with the wide central component (co-spatial to LR:A) slightly redshifted.

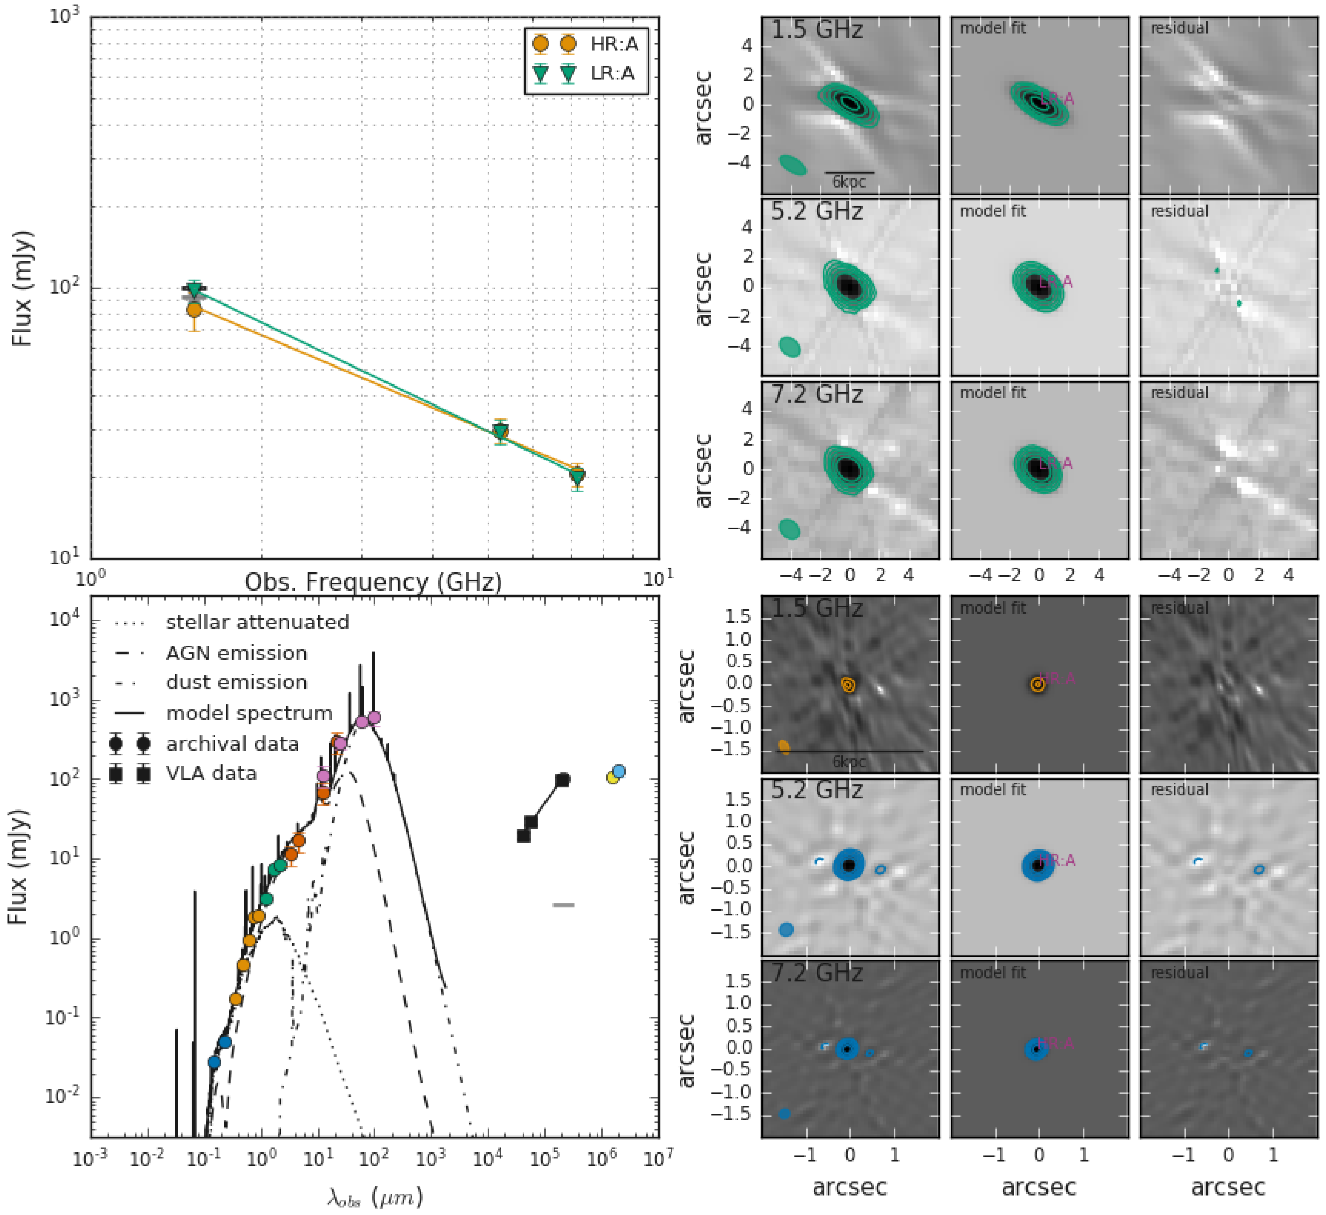


**Figure B13.** Same as Fig. B1 but for J1010+0612. Although there are no morphological features in the radio for this source, the GLEAM and TGSS data suggest either an unusual spectral shape (a peak between 1.4 and 0.15 GHz then rising again; see e.g., Hogan et al. 2015) or variability. A peak within those frequencies would mean a size of 0.2–10.5 kpc according to the turnover - size relation from CSS/GPS sources (Orienti & Dallacasa 2014), consistent with the deconvolved size of 0.2 kpc we measured (see Section 4.1.2).

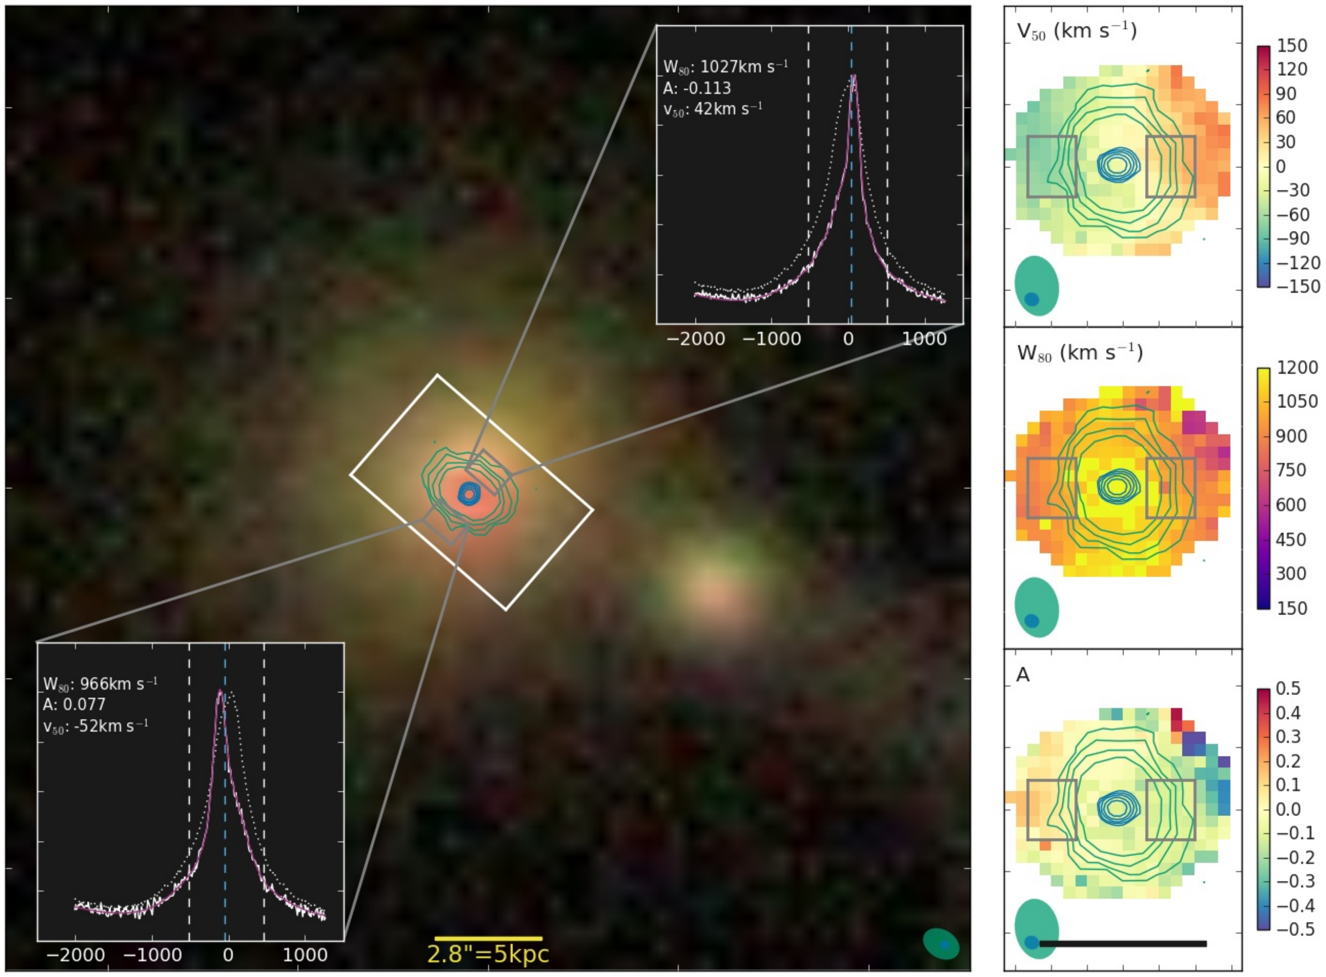


**Figure B14.** As Fig. B2 but for J1010+0612 except with the three-colour SDSS image shown in the main panel. Although there are no morphological features seen in this source at the spatial scales we are sensitive to, the width of the [O III] profile is indicative of fast ($\gtrsim$1000km s$^{-1}$) outflows. However, we do see a tentative alignment between the position angles calculated for the ionized gas and from the radio image (see Section 5.3), suggesting the presence of barely resolved features.

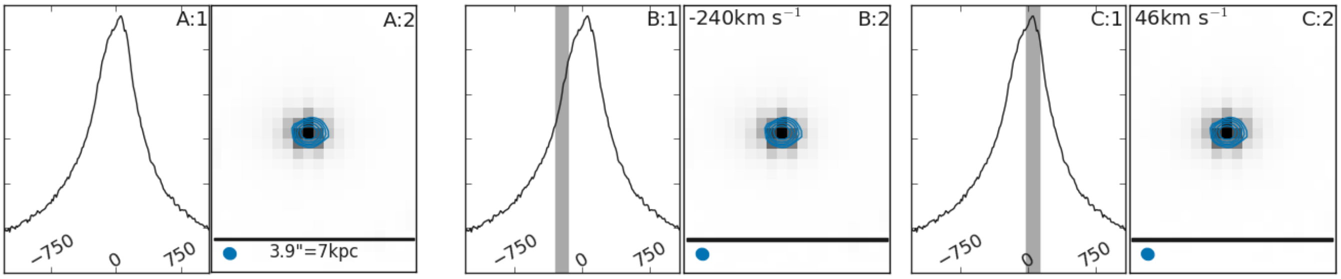


**Figure B15.** Same as Fig. B3 but for J1010+0612.

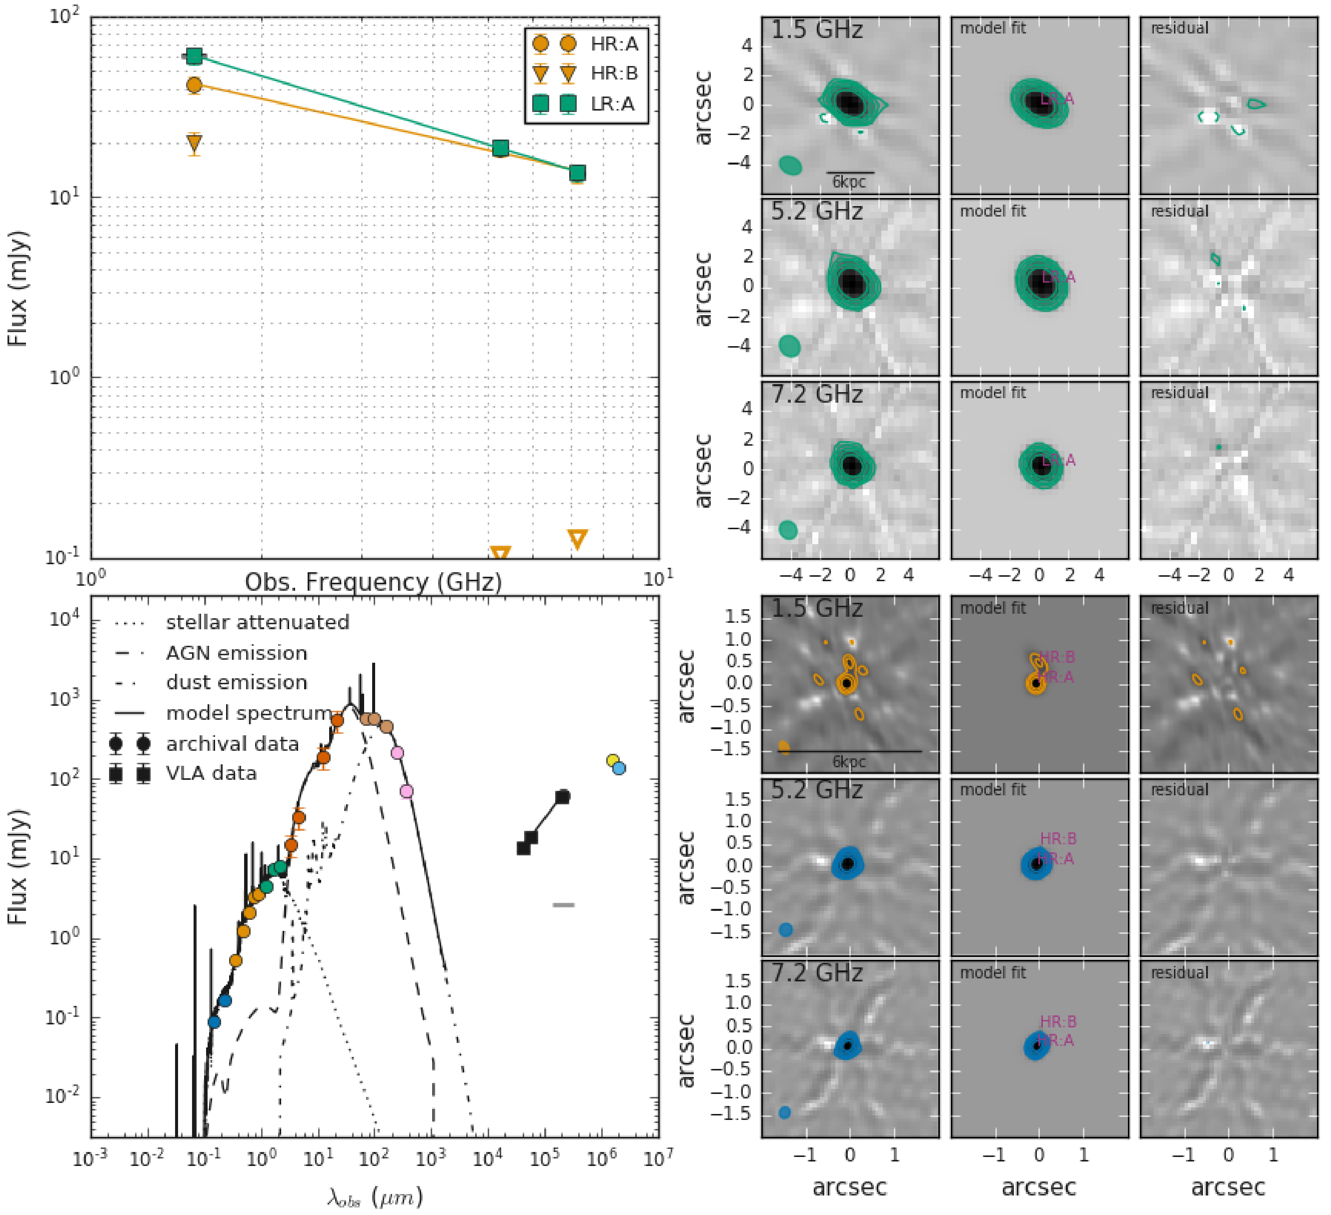


**Figure B16.** Same as Fig. B1 but for J1100+0846. HR:B is only detected in the e-MERLIN data. Although it is a 7$\sigma$ detection in e-MERLIN (see Table 4) and there are wings in the synthesised beam with a similar percentage of the peak flux density, the lack of a symmetric feature in the image suggests this could be real, in which case it would be a highly variable radio structure (see Section 5.2.4). The GLEAM and TGSS data suggest that the radio SED peaks somewhere between 1.4 and 0.14 GHz which would correspond to sizes between 0.2 and 10.5 kpc assuming the source follows the size - turnover frequency relation from CSS and GPS sources (Orienti & Dallacasa 2014). This would be consistent with the 0.8 kpc size measured between HR:A and HR:B.

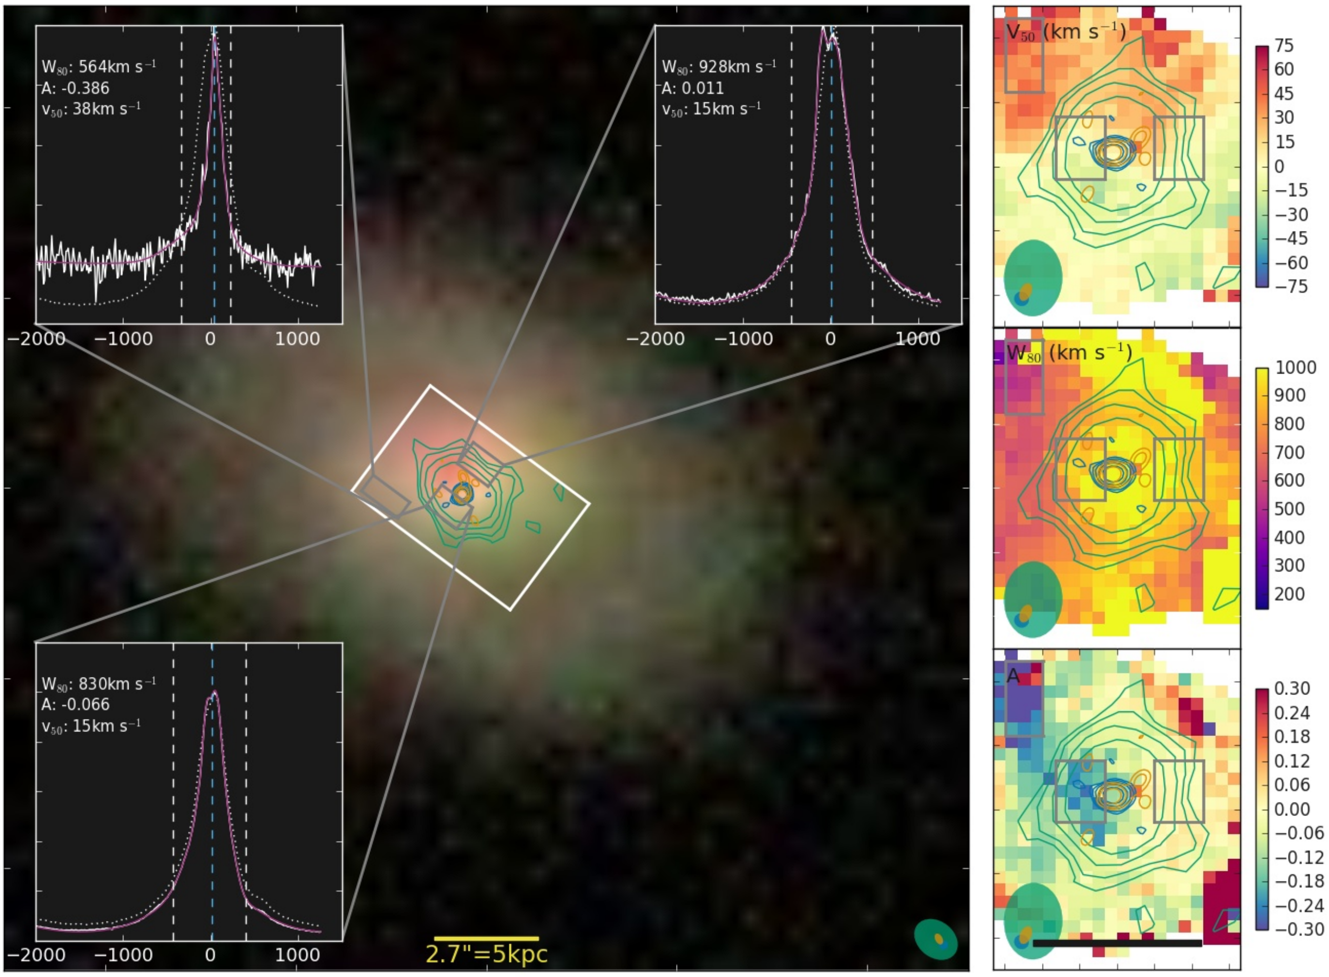


**Figure B17.** Same as Fig. B2 but for J1100+0846, with the the SDSS three-colour image in the main panel. The [O III] emission-line profile in this source is both wide ($W_{80}$≈1000) and disturbed (irregular velocity, width and asymmetry maps). However, we are unable to see a clear connection between the ionized gas kinematics and radio morphology in this source with the current data.

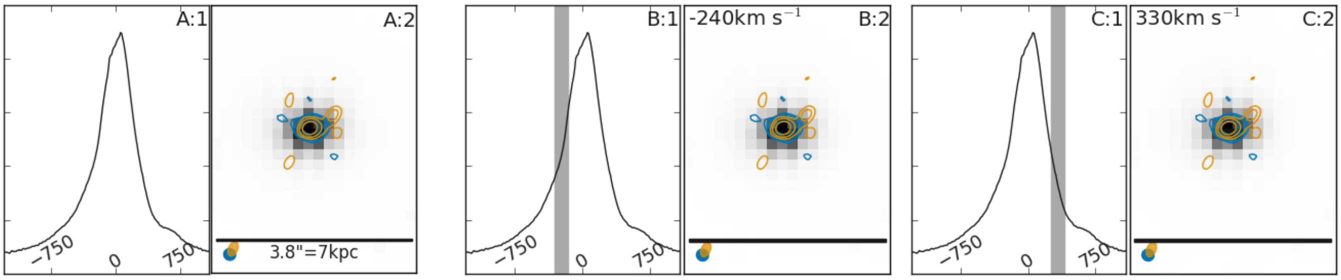


**Figure B18.** As Fig. B3 but for J1100+0846.

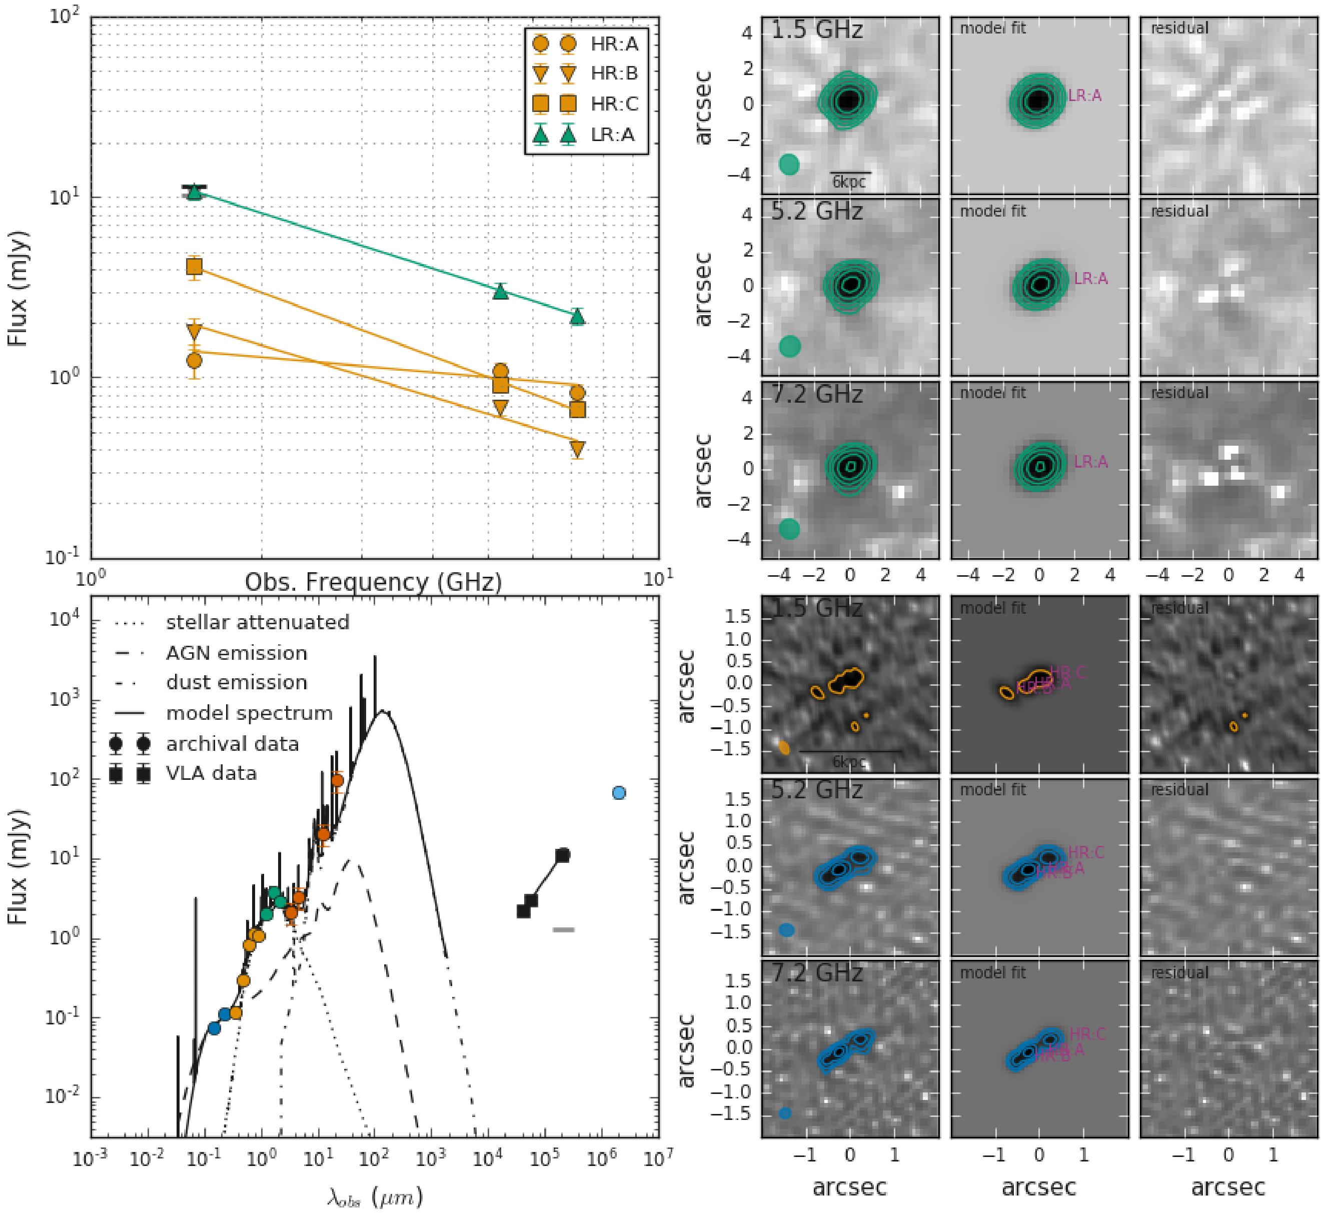


**Figure B19.** Same as Fig. B1 but for J1316+1753. The three morphological features in the high resolution images for this source have a distinctive triple (lobe-core-lobe) morphology. The relative flatness of the spectral index of HR:A ($\alpha = -0.3$) and steepness of the HR:B and HR:C components (each with $\alpha \approx -1$) is consistent with this interpretation.

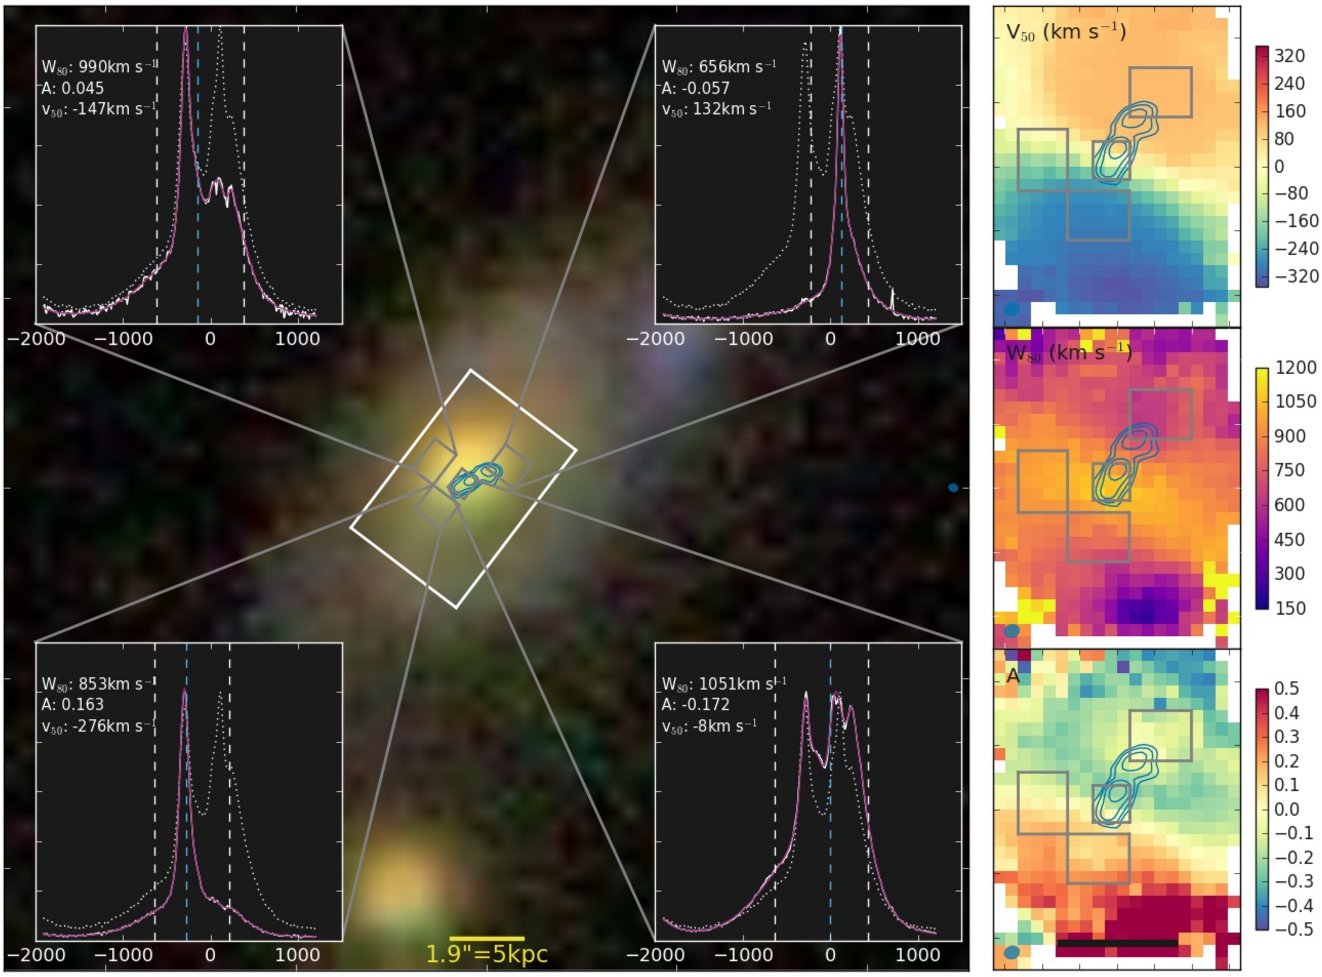


**Figure B20.** As Fig. B2 but for J1316+1753 with the SDSS three-colour image in the main panel. The velocity gradient seen could be a biconical outflow driven by the jets. The outflow interpretation is supported by the large (∼1000 km s$^{-1}$) line widths and the association between the location of the jets and [O III] kinematic components (also see Fig. B21).

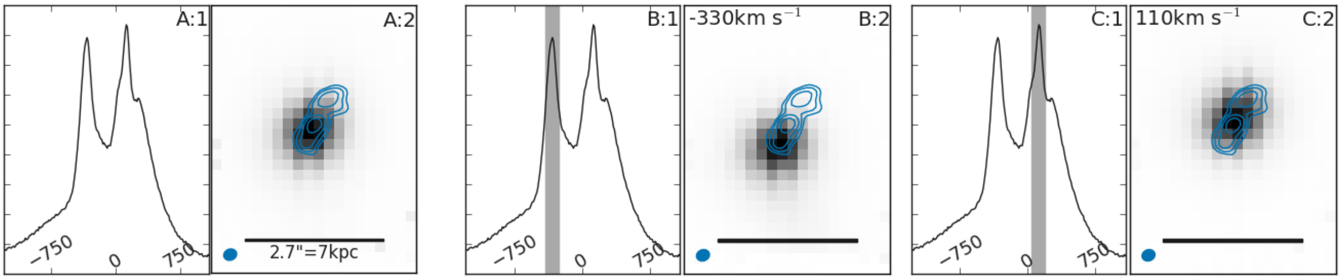


**Figure B21.** As Fig. B3 but for J1316+1753. Panels B and C show that the blue and red [O III] components roughly lie on either side of the radio features.

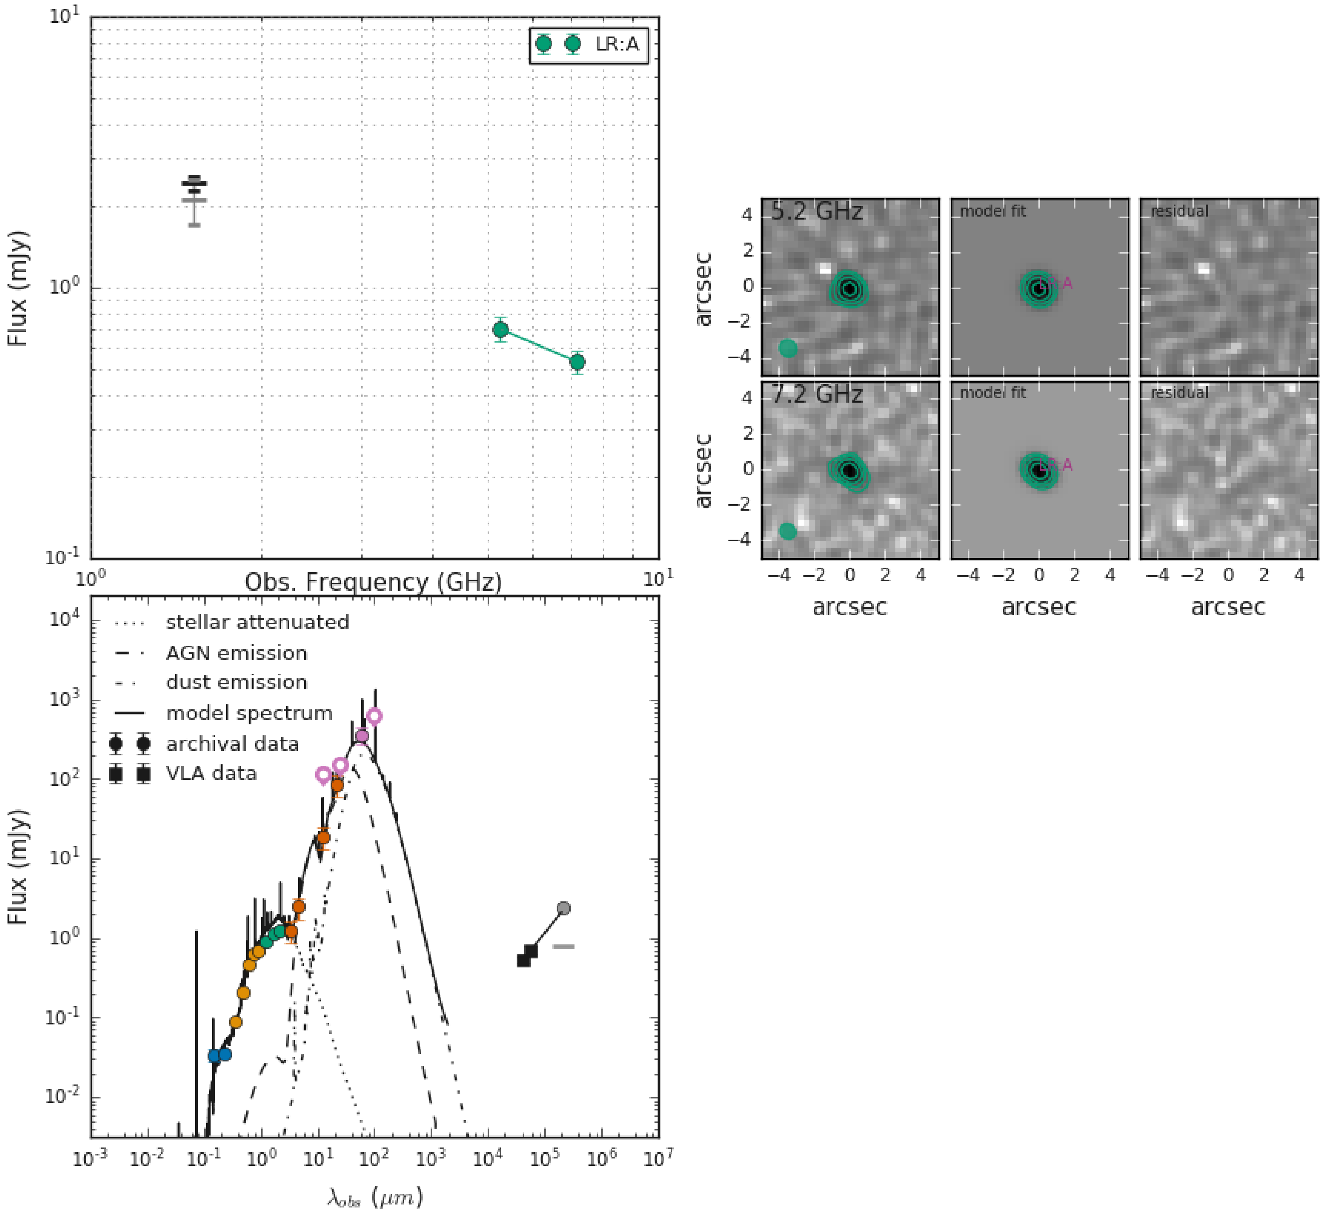


**Figure B22.** Same as Fig. B1 but for J1338+1503. We only have VLA C-band B-configuration data for this object (see Section 3) and hence can not comment on the presence of $\lesssim$kpc scale features similar to what we see in many of the other targets. We see a single morphological component with $\alpha = -0.9$.

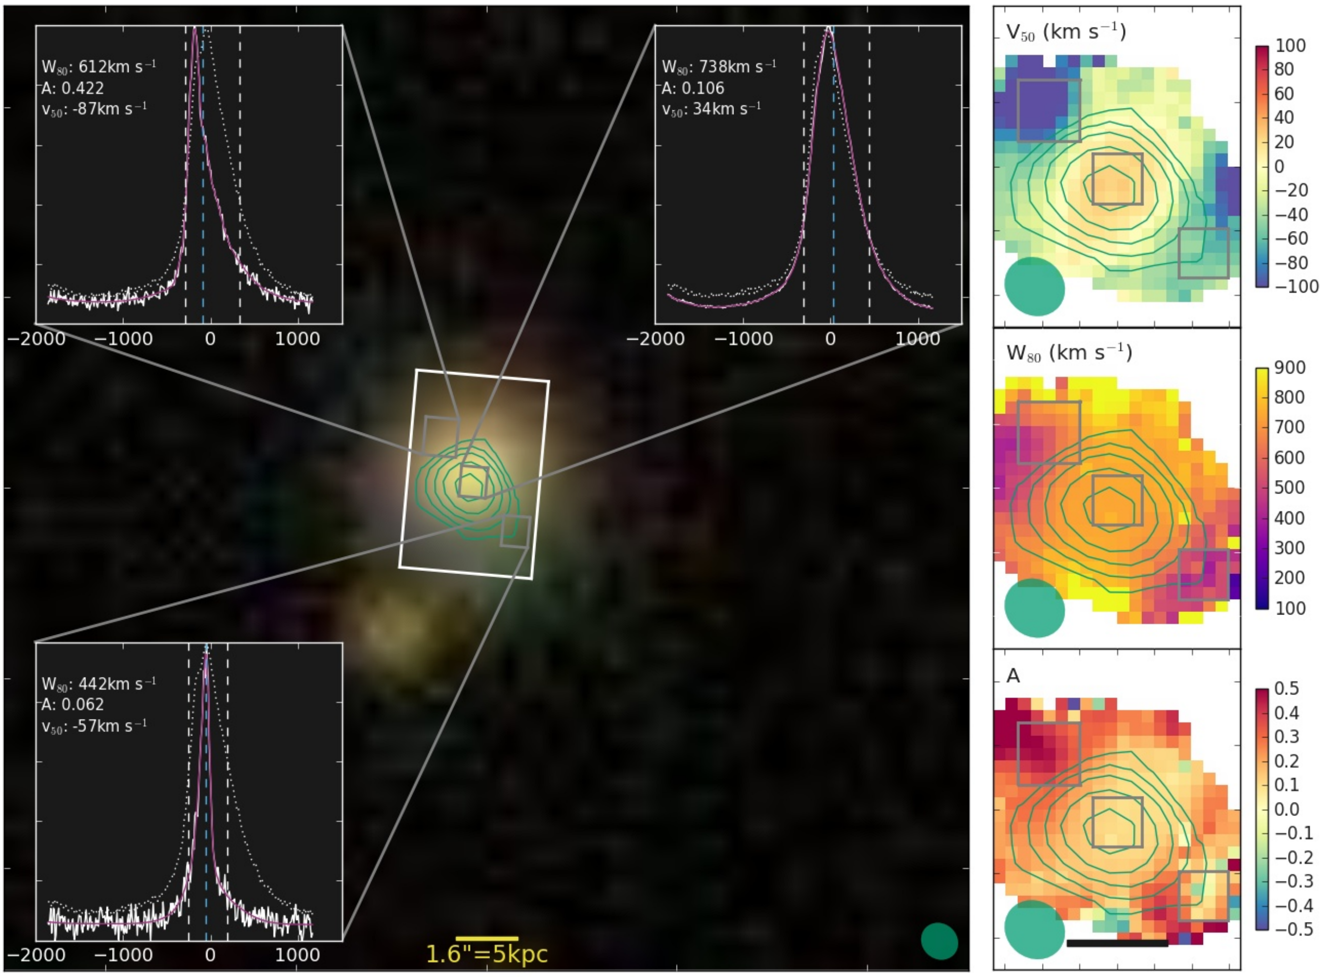


**Figure B23.** As Fig. B2 but for J1338+1503, with the three-colour SDSS image shown in the main panel. The ionized gas in this source is disturbed (seen in the velocity, width and asymmetry maps), possibly related to unresolved jet and/or quasar wind driven outflows. The alignment measured between the radio and [O III] features from our fitting, but not visible by eye (see Section 5.3.1) suggest there might be unresolved radio features in this target.

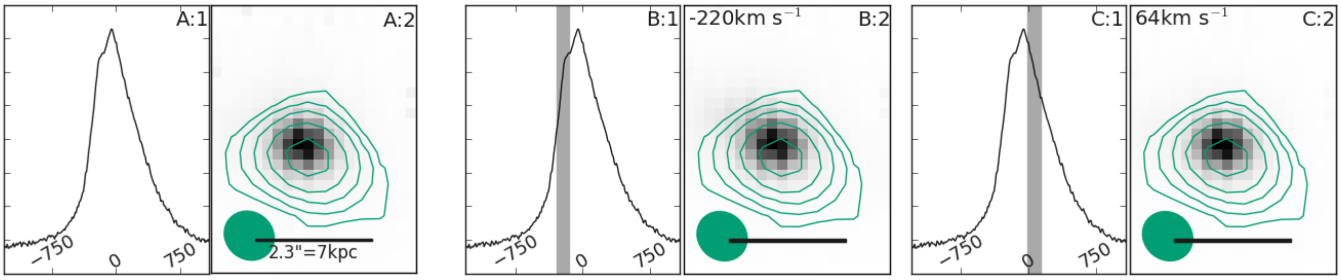


**Figure B24.** Same as Fig. B3 but for J1338+1503.

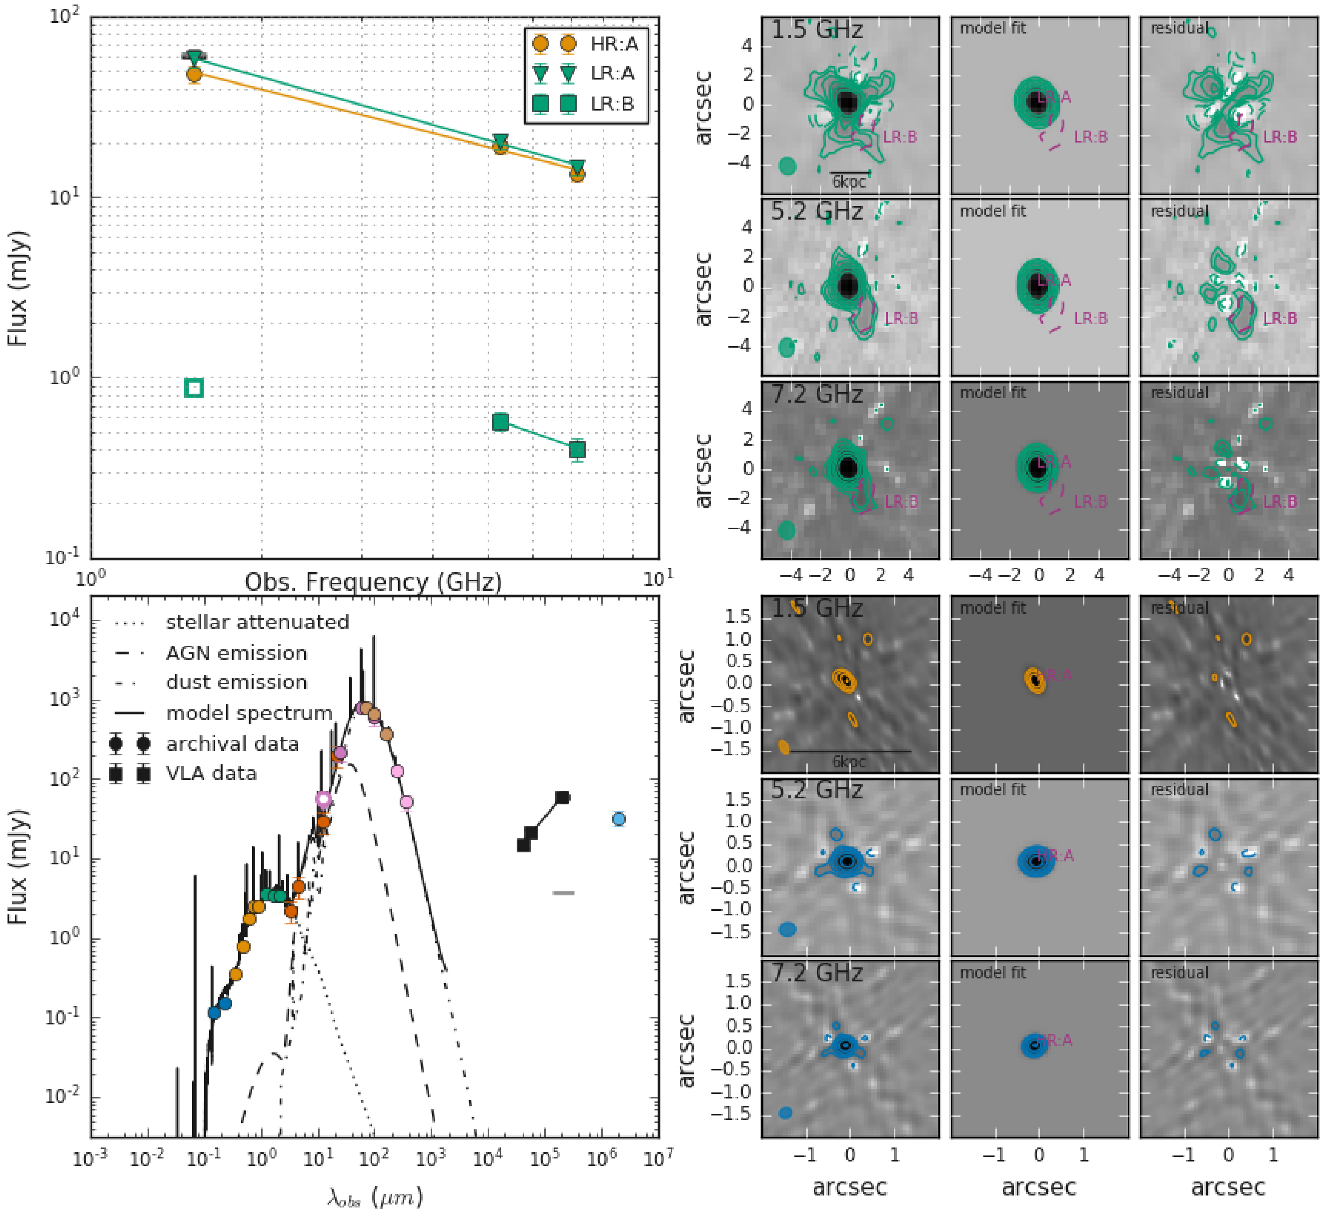


**Figure B25.** Same as Fig. B1 but for J1356+1026. LR:B is a diffuse (not visible in the HR data), steep spectrum ($\alpha$ = −1.1) component whose exact nature is unclear but which might be a deflected jet or a tail of star formation (see Section 5.2.4). The nuclear component (HR:A / LR:A) also has a steep spectrum ($\alpha \approx -0.8$), which may suggest that the nuclear component contains a still unresolved jet. Furthermore, the turnover in the radio SED (which is dominated by the nuclear HR:A component), implies a size between 0.2 and 10 kpc, assuming the size – turnover frequency relation from Orienti & Dallacasa 2014), consistent with the deconvolved size measured in Section 4.1.2 (0.3 kpc).

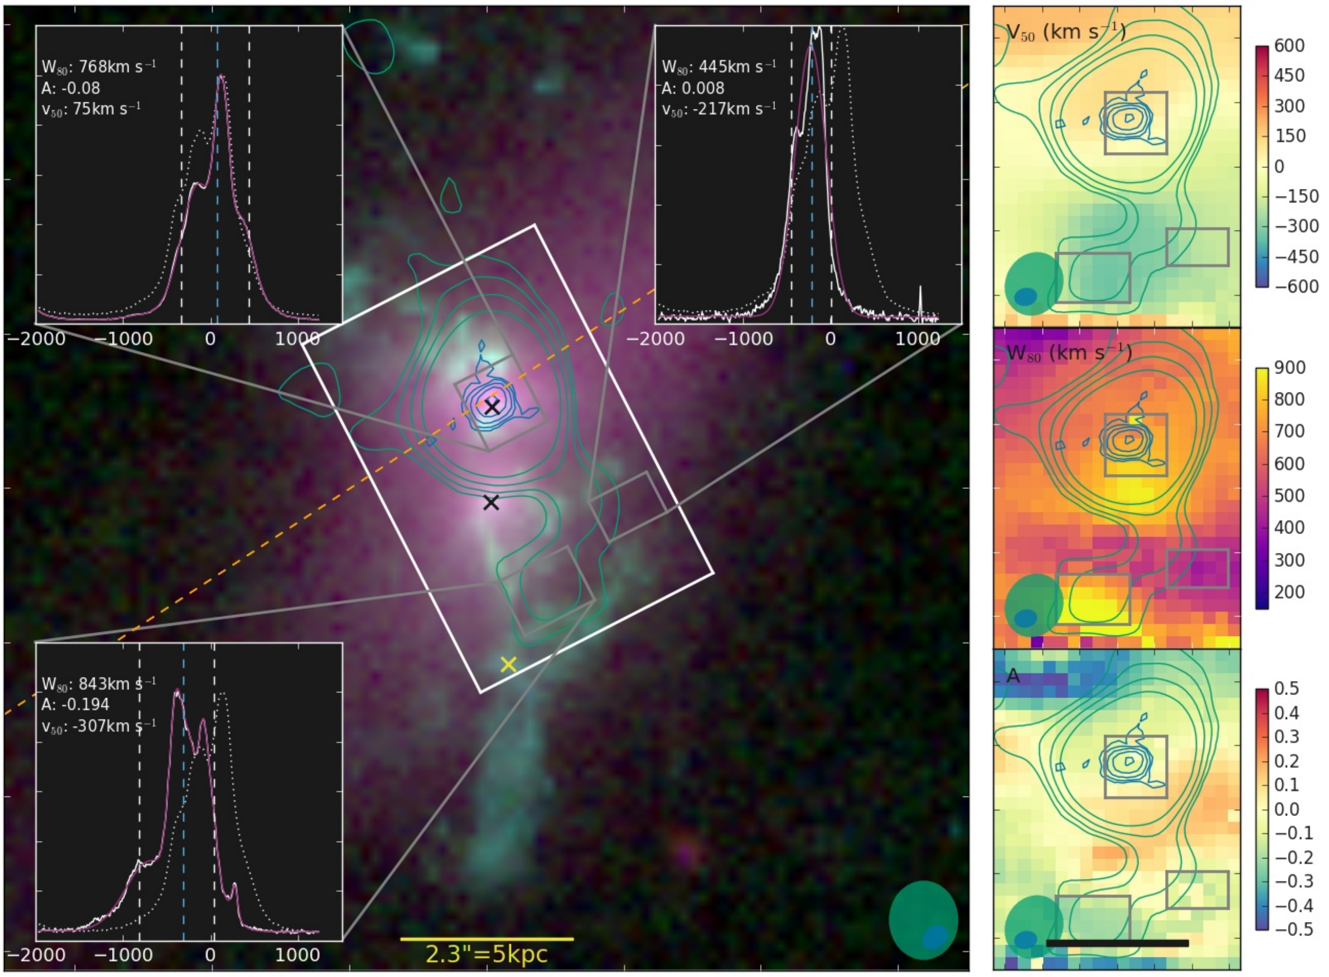


**Figure B26.** Same as Fig. B2 but for J1356+1026. The background image is from archival HST data with F160W (continuum) in red, the F814W filter (mix of H$\alpha$ and continuum) in blue and the F438W ([O II] dominated) filter in green (Comerford et al. 2015). This source has been identified to host two AGN, which are marked by black x's with their locations taken from the peaks in the F814W image. The yellow x marks the approximate position of the base of the quasi-spherical outflow / bubble identified by Greene et al. (2012), that is not covered by our GMOS observations. LR:B terminates just at the base of the bubble, suggesting the two features could be related. The lack of line emission coincident with LR:B challenges its interpretation as due to star formation. The orange dashed line marks the direction of the velocity gradient in the cold gas disc from ALMA data (Sun et al. 2014).

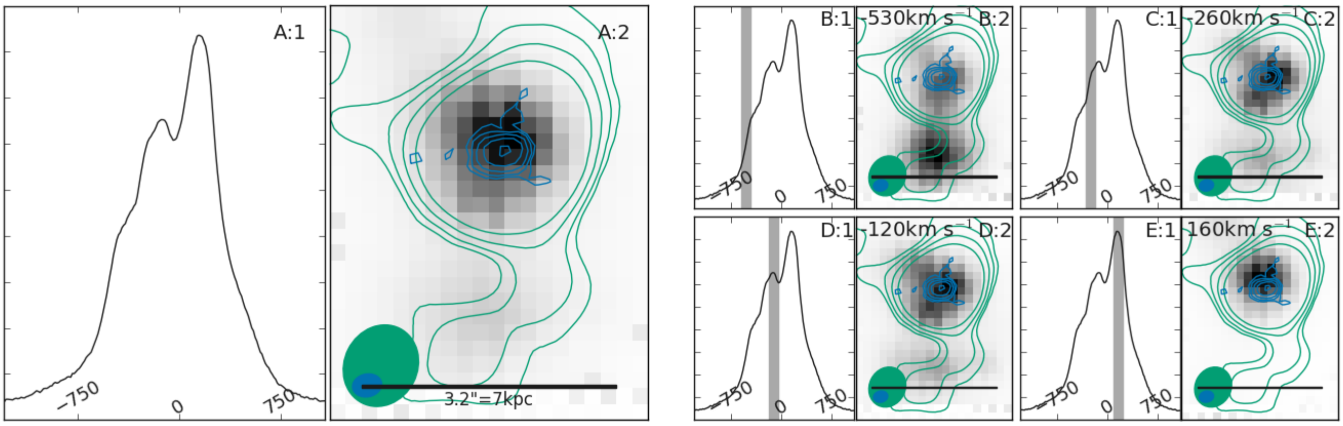


**Figure B27.** As Fig. B3 but for J1356+1026. Panel B shows that the broad [O III] emission in the vicinity of the extended radio structure is kinematically distinct from the rest of the ionized gas, potentially due to interactions with a jet. Panels C and D show that the prominent blue wing in the emission-line profile is mostly associated with a region of [O III] emission extended to the north east of the brightest nuclei.

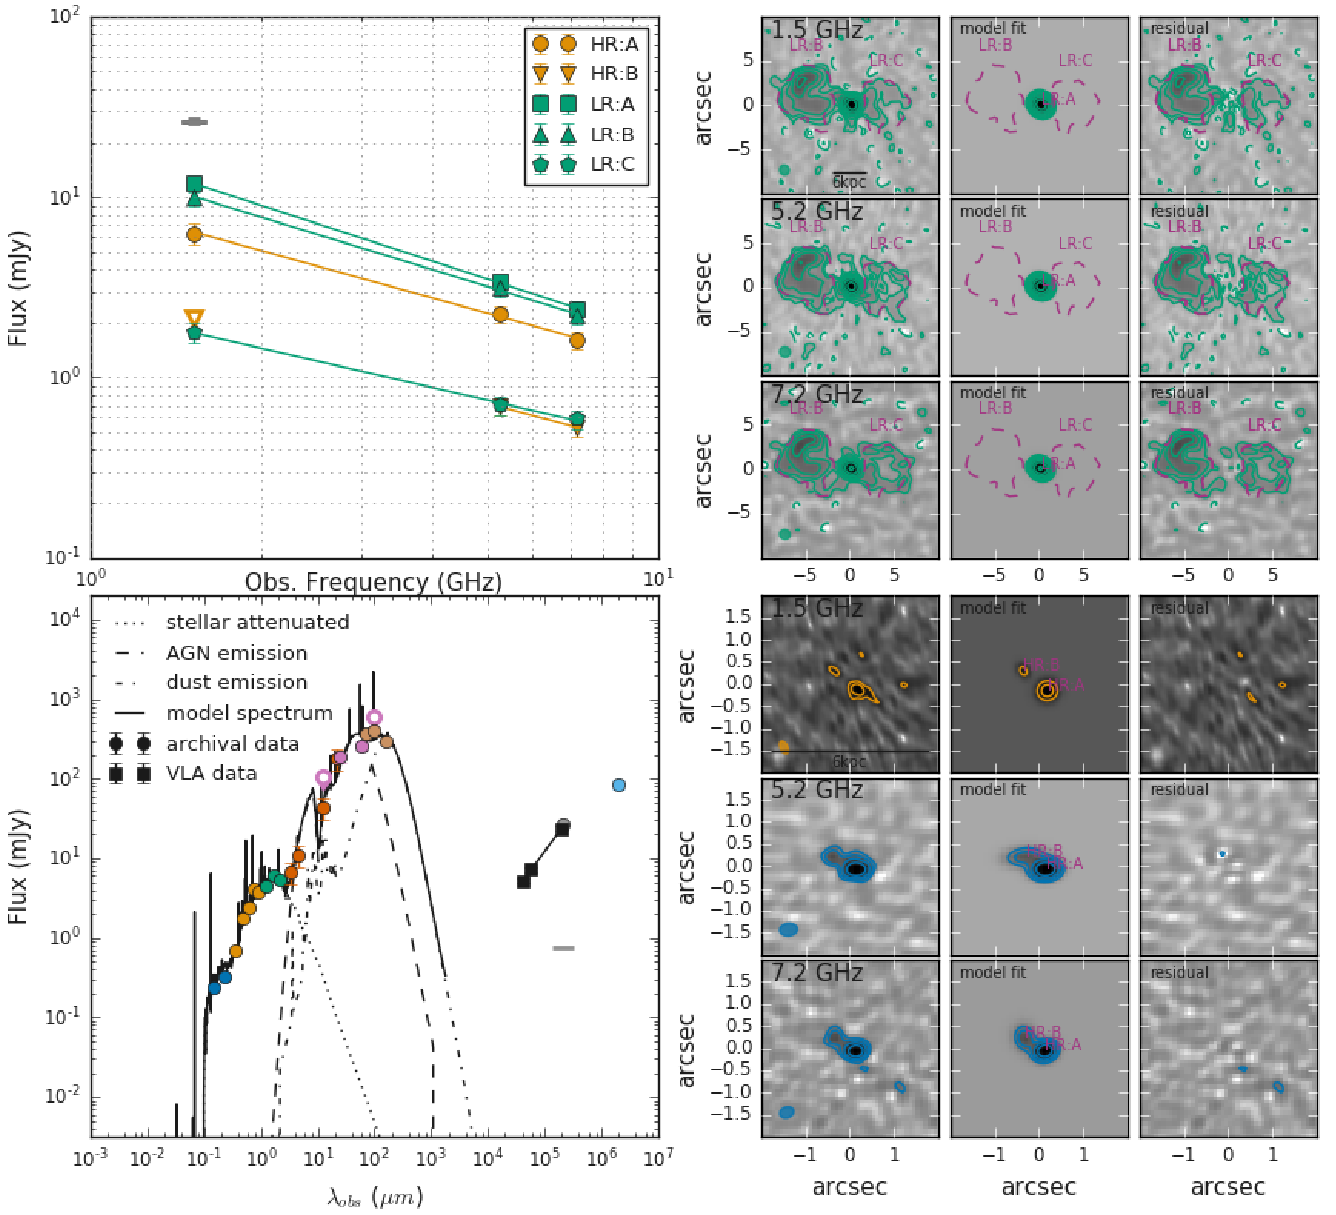


**Figure B28.** Same as Fig. B1 but for J1430+1339. The hollow radio bubbles seen in this source (LR:B and LR:C) are unique among this sample. HR:A and HR:B could be compact (LLS=0.8 kpc) radio jet/lobes. All of the radio components have steep spectral indices ($-0.7 < \alpha < -1$).

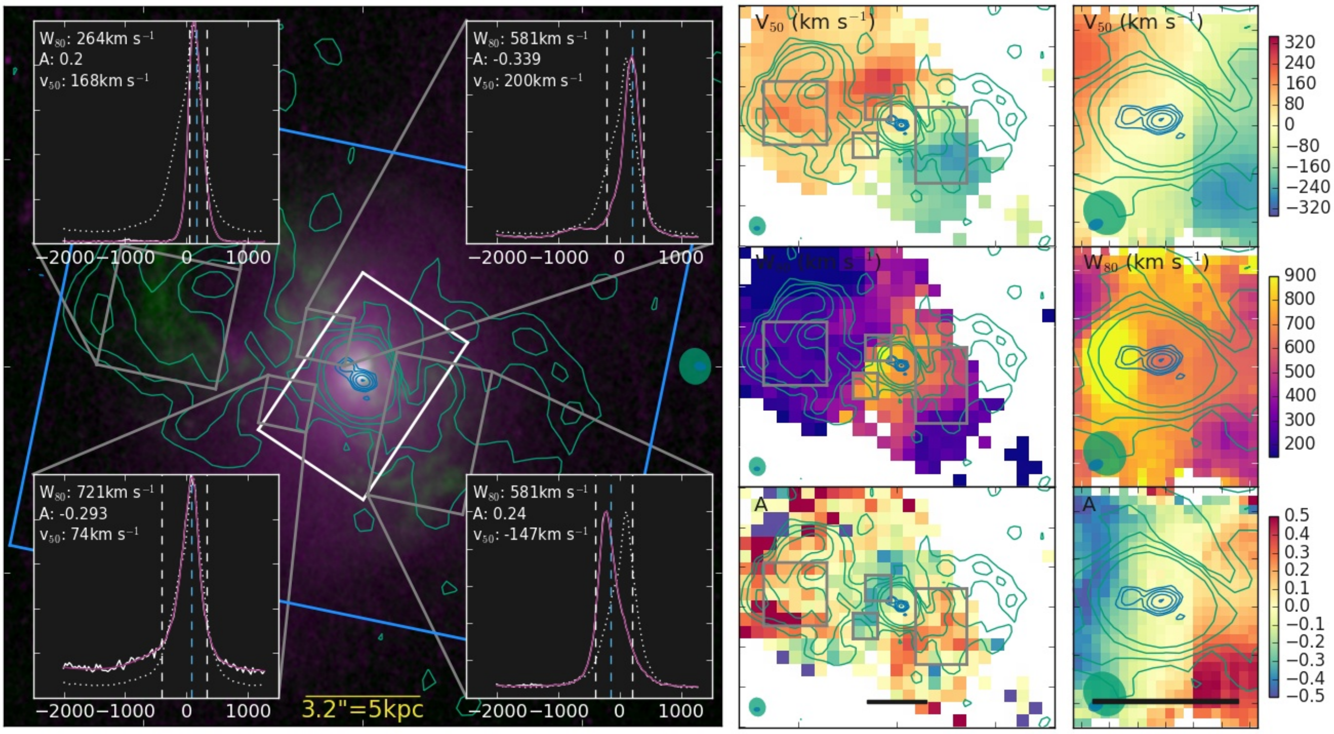


**Figure B29.** Same as Fig. B2 but for J1430+1339. The background image is from archival HST data (continuum in purple and H$\alpha$ in green Keel et al. 2015). As was identified in Harrison et al. (2015) the radio bubbles (LR:B and LR:C) are coincident with similarly shaped structures in the ionized gas each with a distinct velocity (better seen in Fig. B30). It has also been identified that the bubbles are bright in soft X-rays, whose spectrum is consistent with shocked gas (Lansbury et al. 2018). There is a wide and blue shifted ionized gas component, indicative of an outflow, just beyond HR:B (shown in the top right [O III] line profile). This source is discussed in more detail in Harrison et al. (2015).

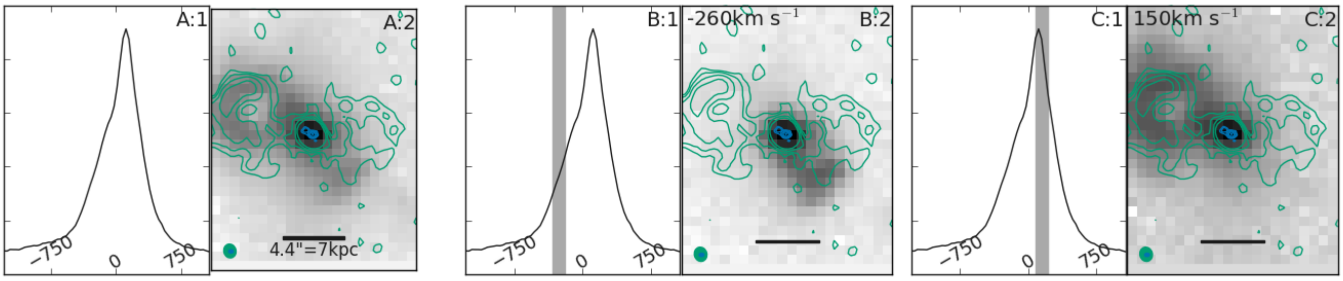


**Figure B30.** As Fig. B3 but for J1430+1339. The ionized gas components coincident with the radio bubbles are kinematically distinct (also see Villar-Martín et al. 2018).

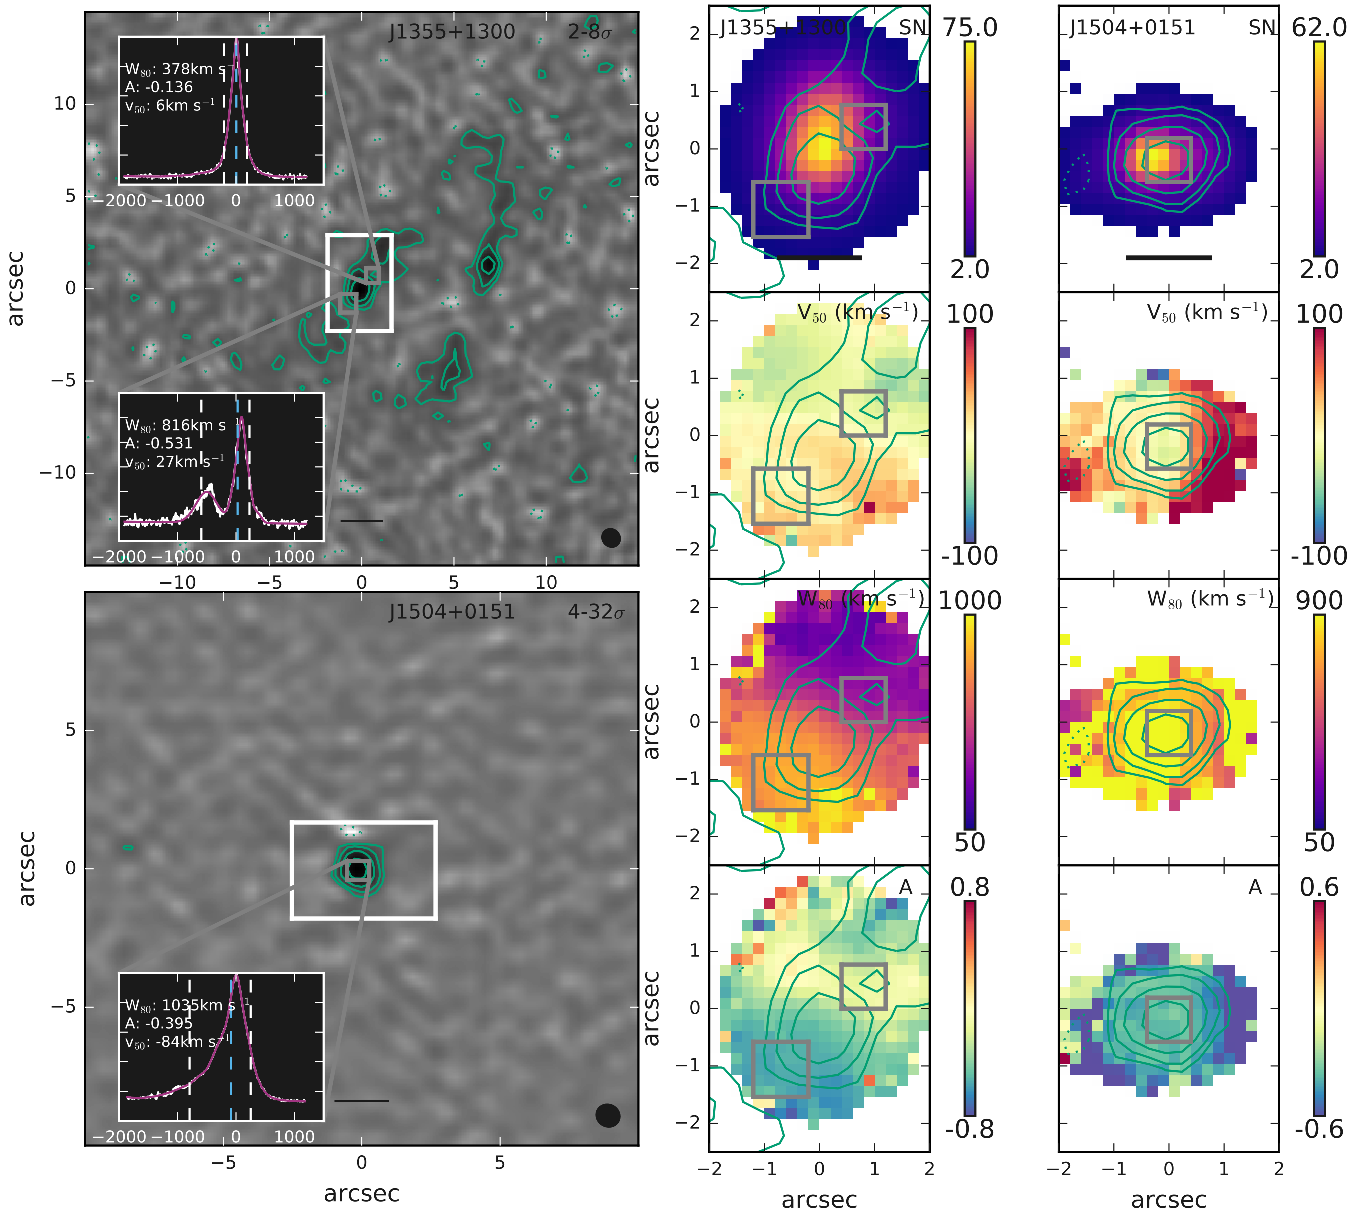


**Figure C1.** Our VLA and GMOS IFS data for the two AGN in the original Harrison et al. (2014) sample for which we have VLA C-band B-configuration data but which were not in the primary sample discussed here. The left column contains the VLA images for each (the details of which are in Table B1), and the black scale bar in the bottom centre represents 6 kpc. A white rectangle marks the GMOS FOV and the [O III] emission-line profiles shown in various corners are extracted from the regions shown in grey boxes. The weighted average of the spaxels included is shown in white with the fit in magenta; the vertical white dashed lines mark $v_{10}$ and $v_{90}$ with the light blue dashed line showing $v_{50}$, which is also written, along with the $W_{80}$ and asymmetry for the extracted [O III] line profile in the top left of each line profile overlay (see Section 4.2 for parameter definitions). The second and third columns show the GMOS maps of S/N, $v_{50}$, $W_{80}$ and A with the boxes used for the extracted line profiles overlaid, the scale bar in S/N image for each source is the same as in the main panel. There is not much of note in either the radio or IFS data for J1504+0151 except that the wide [O III] line (~900 km s$^{-1}$) suggest the presence of an outflow. Our radio images for J1355+1300 however reveal extensive possibly jet-like features which seem to be aligned with kinematic features seen in our IFS data, although the GMOS FOV is smaller than the radio features seen. In particular we see line splitting in the south-east corner possibly related to a jet-launched bubble, similar to that seen in J1000+1242 and J1356+1026. We have no spectroscopic information for the extended radio features seen to the west in J1355+1300, so cannot comment if it is related or a background source.
